# Supplementary material for: Hypothesis Testing for Functional Linear Models via Bootstrapping
Source: arXiv:2109.02309 source file (2024-04-01)
Supplement: Supplementary file 1 [file iFLR-supp.pdf]

# Supplementary Material for “A Unified Approach to Hypothesis Testing for Functional Linear Models”

Yinan Lin and Zhenhua Lin

Department of Statistics and Data Science, National University of Singapore

**Organization.** In Section S1, we provide a mean model related to the test statistic, preparing for the proofs of Theorems 3.5–3.7. The proofs of these theorems are given in Sections S2 and S3. Section S4 is devoted to proofs for Theorems 3.8 and 3.9. Some auxiliary results used in the proofs are collected in Section S5. In Section S6, we prove Proposition 2.1. In Section S7 we presents a proof for Proposition 3.4, which depends on a concentration inequality established in Section S8.

**Notations and conventions.** Recall the following eigendecomposition for the covariance operators

$$C_X = \sum_{j_1=1}^{\infty} \lambda_{j_1} \phi_{j_1} \otimes \phi_{j_1}, \quad C_Y = \sum_{j_2=1}^{\infty} \rho_{j_2} \psi_{j_2} \otimes \psi_{j_2}, \quad (\text{S1})$$

and the Karhunen-Loève expansions

$$X_i = \sum_{j=1}^{\infty} \langle X_i, \phi_j \rangle \phi_j = \sum_{j=1}^{\infty} \sqrt{\lambda_j} \eta_{ij}^X \phi_j \in \mathcal{X}, \quad Y_i = \sum_{j=1}^{\infty} \langle Y_i, \psi_j \rangle \psi_j = \sum_{j=1}^{\infty} \sqrt{\rho_j} \eta_{ij}^Y \psi_j \in \mathcal{Y},$$

where  $\eta_{ij}^X$ s (also for  $\eta_{ij}^Y$ s) are zero-mean random variables with unit variance, and uncorrelated with each other for each  $i, j$ . The variance of the random variable  $\langle X_i, \phi_{j_1} \rangle$  is  $\lambda_{j_1}$  for each  $i, j_1$ , while the variance of the random variables  $\langle Y_i, \psi_{j_2} \rangle$  is  $\rho_{j_2}$  for each  $i$  and  $j_2$ . In addition, for the error term  $Z$ , we have the following expansions

$$C_Z = \mathbb{E}[Z \otimes Z] = \sum_{j=1}^{\infty} \kappa_j \theta_j \otimes \theta_j, \quad Z_i = \sum_{j=1}^{\infty} \sqrt{\kappa_j} \eta_{ij}^Z \theta_j \in \mathcal{Y},$$

and let

$$\tilde{Z}_{ij} = \langle Z_i, \psi_j \rangle, \quad \tilde{\kappa}_j = \mathbb{E} \tilde{Z}_{ij}^2.$$

For a sequence  $\{c_j\}$ ,  $c_{(j)}$  refers to the decreasingly ordered entries in this sequence. In addition,  $(j)$  denotes the index of  $c_{(j)}$  in the original sequence  $\{c_j\}$ . When there are multiple sequences, we may also use the symbols  $(j)_1$  and  $(j)_2$  for indices in different sequences. For example, for  $\{\lambda_{j_1}\}_{j_1=1}^{\infty}$  and  $\{\rho_{j_2}\}_{j_2=1}^{\infty}$ , we denote by  $\{\lambda_{(j_1)_1}\}$  the decreasingly ordered sequence of  $\{\lambda_{j_1}\}_{j_1=1}^{\infty}$  and by  $\{\rho_{(j_2)_2}\}$  the decreasingly ordered

sequence of  $\{\rho_{j_2}\}_{j_2=1}^\infty$ .

Unless otherwise stated, quantities depending on  $(\tilde{\phi}, \tilde{\psi})$  are marked by the tilde symbol, while those without the tilde mark depend on  $(\phi, \psi)$ . For example,  $\tilde{V}_i = V_i(\tilde{\phi}, \tilde{\psi})$  and  $V_i = V_i(\phi, \psi)$ . We may also use the symbol like  $\hat{\sigma} = \hat{\sigma}(\tilde{\phi}, \tilde{\psi})$  to indicate that it is an empirical quantity related to  $(\tilde{\phi}, \tilde{\psi})$ . We primarily focus on the case that  $d_{\mathcal{X}} = d_{\mathcal{Y}} = \infty$ ; the case that either of  $d_{\mathcal{X}}$  and  $d_{\mathcal{Y}}$  is finite is simpler and can be analyzed in an almost identical fashion.

Finally, let  $\mathbb{N}$  denote the set of natural numbers. For  $j_1 \geq 1$  and  $j_2 \geq 1$ , let  $\xi_{ij_1} = \langle X_i, \phi_{j_1} \rangle_1$  and  $\zeta_{ij_2} = \langle Y_i, \psi_{j_2} \rangle_2$ ; the subscripts of the inner products are sometimes omitted when they are clear from the context. For  $j \in \{1, \dots, p_1 p_2\}$ , the  $j$ th element of  $V_i = \xi_{ij_1} \zeta_{ij_2}$  is determined by the basis functions  $\phi_{j_1}$  and  $\psi_{j_2}$  for some  $j_1 \in \{1, \dots, p_1\}$  and  $j_2 \in \{1, \dots, p_2\}$  such that  $j = p_1(j_2 - 1) + j_1$ . For the infinite sequence  $V_i^\infty = \xi_{ij_1} \zeta_{ij_2}$  for  $j_1 \in \mathbb{N}$  and  $j_2 \in \mathbb{N}$ , we use  $(j_1, j_2) \in \mathbb{N}^2$  to indicate the position of  $\xi_{ij_1} \zeta_{ij_2}$  in  $V_i^\infty$ . Such indexing is also applied to  $\tilde{V}_i$  and  $\tilde{V}_i^\infty$  as well as other related series such as the expected values of  $\tilde{V}_i$  and  $\tilde{V}_i^\infty$ .

## S1 A Mean Model Related to the Test

In Section 3, we present three uniform approximation results related to the test statistics, namely, the Gaussian approximation, the bootstrap approximation and the approximation with empirical variances, uniformly over the class  $\mathcal{F}_p$ .

Before presenting the proofs of these theorems, we represent  $V_i(\phi, \psi) := V_i = (\xi_{ij_1} \zeta_{ij_2}, j_1 = 1, \dots, p_1, j_2 = 1, \dots, p_2) \in \mathbb{R}^p$ , the truncated version of  $V_i^\infty$ , by a mean model first, where  $\xi_{ij_1} = \langle X_i, \phi_{j_1} \rangle_1$ ,  $\zeta_{ij_2} = \langle Y_i, \psi_{j_2} \rangle_2$  and  $p = p_1 p_2$ . Specifically, we write

$$V_i = \nu + \Sigma^{\frac{1}{2}} \varepsilon_i, \quad i = 1, \dots, n,$$

where  $\varepsilon_i = \Sigma^{-\frac{1}{2}} \epsilon_i$ ,  $\epsilon_i = (\epsilon_{i,1}, \dots, \epsilon_{i,p})$  and

$$\epsilon_{i,j} = \langle X_i, \phi_{j_1} \rangle \langle Y_i, \psi_{j_2} \rangle - \mathbb{E}[\langle X_i, \phi_{j_1} \rangle \langle Y_i, \psi_{j_2} \rangle], \quad i = 1, \dots, n,$$

for  $j = p_1(j_2 - 1) + j_1$  and  $p = p_1 p_2$ . In this representation,  $\mathbb{E} \epsilon_i = 0$  and denote  $\Sigma = \mathbb{E}[\epsilon_i \epsilon_i^\top]$ . Moreover,  $\mathbb{E}[\varepsilon_i \varepsilon_i^\top] = I_p$ .

When the basis  $(\tilde{\phi}, \tilde{\psi})$  is used, we have a similar representation

$$\tilde{V}_i = \tilde{\nu} + \tilde{\Sigma}^{\frac{1}{2}} \tilde{\varepsilon}_i, \quad i = 1, \dots, n, \tag{S2}$$

where  $\tilde{\nu} = \mathbb{E} \tilde{V}_1$  is the mean vector of  $\tilde{V}_1$ ,  $\tilde{\Sigma} = \text{Var}(\tilde{V}_1) = \mathbb{E}[(\tilde{V}_1 - \tilde{\nu})(\tilde{V}_1 - \tilde{\nu})^\top]$  is the covariance matrix of  $\tilde{V}_1$ ,  $\tilde{\varepsilon}_i = \tilde{\Sigma}^{-\frac{1}{2}} \tilde{\epsilon}_i$ ,  $\tilde{\epsilon}_i = (\tilde{\epsilon}_{i,1}, \dots, \tilde{\epsilon}_{i,p})$ ,  $\tilde{\Sigma}^{-\frac{1}{2}}$  is the square-root of the pseudo-inverse of  $\tilde{\Sigma}$  (the existence is guaranteed

due to the symmetry and the positive semi-definiteness of  $\tilde{\Sigma}$ ), and

$$\tilde{\epsilon}_{i,j} = \langle X_i, \tilde{\phi}_{j_1} \rangle \langle Y_i, \tilde{\psi}_{j_2} \rangle - \mathbb{E}[\langle X_i, \tilde{\phi}_{j_1} \rangle \langle Y_i, \tilde{\psi}_{j_2} \rangle], \quad i = 1, \dots, n.$$

In this representation, we also have  $\mathbb{E}\tilde{\epsilon}_i = 0$  and  $\mathbb{E}[\tilde{\epsilon}_i \tilde{\epsilon}_i^\top] = \tilde{\Sigma}$  as well as  $\mathbb{E}[\tilde{\epsilon}_i \tilde{\epsilon}_i^\top] = I_r$ , where  $r$  is the rank of  $\tilde{\Sigma}$ .

## S2 Proofs of Theorem 3.5 and Theorem 3.7

*Proof.* With the help of Propositions S2.1, S2.2 and S2.4, we can apply the approximation results in Lopes and Yao (2022) and Lin et al. (2022) on  $\tilde{V}$  and related analogs. Therefore, for each  $(\tilde{\phi}, \tilde{\psi}) \in \mathcal{F}_p$ , we have

$$d_K(\mathcal{L}(M(\tilde{\phi}, \tilde{\psi})) - \mathcal{L}(\check{M}(\tilde{\phi}, \tilde{\psi}))) \leq c_1 n^{-\frac{1}{2} + \delta},$$

and

$$d_K(\mathcal{L}(\hat{M}(\tilde{\phi}, \tilde{\psi})) - \mathcal{L}(M(\tilde{\phi}, \tilde{\psi}))) \leq c_2 n^{-\frac{1}{2} + \delta}.$$

Moreover, if we go through the proof details of these propositions, the right-hand sides of both equations are not dependent on  $(\tilde{\phi}, \tilde{\psi})$ , i.e., the *same* constants  $c_1 > 0$  and  $c_2 > 0$  are shared among  $(\tilde{\phi}, \tilde{\psi})$ . Consequently, we conclude that

$$\sup_{(\tilde{\phi}, \tilde{\psi}) \in \mathcal{F}_p} d_K(\mathcal{L}(M(\tilde{\phi}, \tilde{\psi})) - \mathcal{L}(\check{M}(\tilde{\phi}, \tilde{\psi}))) \lesssim n^{-\frac{1}{2} + \delta},$$

and

$$\sup_{(\tilde{\phi}, \tilde{\psi}) \in \mathcal{F}_p} d_K(\mathcal{L}(\hat{M}(\tilde{\phi}, \tilde{\psi})) - \mathcal{L}(M(\tilde{\phi}, \tilde{\psi}))) \lesssim n^{-\frac{1}{2} + \delta}.$$

□

The following proposition establishes sub-exponentiality of  $\tilde{\epsilon}_1$  under Assumption 3.1.

**Proposition S2.1.** *With Assumption 3.1,  $\tilde{\epsilon}_1$  from (S2) is a sub-exponential random vector with dimension  $p$ . Specifically, for a constant  $K'$  not depending on  $(\tilde{\phi}, \tilde{\psi})$ ,*

$$\sup_{t \in \mathbb{R}^p, \|t\|_2=1} \|\langle \tilde{\epsilon}_1, t \rangle\|_{\psi_1} \leq K'.$$

*Proof.* By Proposition S5.4, there is a unitary operator  $\tilde{W}$  such that  $\tilde{V}_i^\infty = \tilde{W}^\dagger V_i^\infty$ , where  $\tilde{W}^\dagger$  is the adjoint of  $\tilde{W}$ . Similarly, we also have  $\tilde{\nu}^\infty = \tilde{W}^\dagger \nu^\infty$ . Define  $\epsilon_i^\infty = V_i^\infty - \nu^\infty$  and  $\tilde{\epsilon}_i^\infty = \tilde{V}_i^\infty - \tilde{\nu}^\infty$ . It is seen that

$$\tilde{\epsilon}_i^\infty = \tilde{V}_i^\infty - \tilde{\nu}^\infty = \tilde{W}^\dagger (V_i^\infty - \nu^\infty) = \tilde{W}^\dagger \epsilon_i^\infty,$$

due to the linearity of  $\tilde{W}^\dagger$ . By definition,  $C_\epsilon = \mathbb{E}[\epsilon_i^\infty \otimes \epsilon_i^\infty] = C_V$ , where  $C_V$  is the covariance operator of  $V_i^\infty$  defined in Assumption 3.1. Thus, for any  $t^\infty \in \ell^2$ , according to Assumption 3.1 and the centering inequality

for the sub-exponential random variable (Exercise 2.7.10 in [Vershynin \(2018\)](#)), there exists a constant  $K' > 0$ , such that

$$\|\langle \epsilon_1^\infty, t^\infty \rangle\|_{\psi_1} \leq K' \langle C_\epsilon t^\infty, t^\infty \rangle^{\frac{1}{2}} = K' \left( \mathbb{E} \langle \epsilon_1^\infty, t^\infty \rangle^2 \right)^{\frac{1}{2}}.$$

Moreover,

$$\begin{aligned} \|\langle \tilde{\epsilon}_1^\infty, t^\infty \rangle\|_{\psi_1} &= \|\langle \tilde{W}^\dagger \epsilon_1^\infty, t^\infty \rangle\|_{\psi_1} = \|\langle \epsilon_1^\infty, (\tilde{W}^\dagger)^\dagger t^\infty \rangle\|_{\psi_1} \\ &\leq K' \left( \mathbb{E} \langle \epsilon_1^\infty, (\tilde{W}^\dagger)^\dagger t^\infty \rangle^2 \right)^{\frac{1}{2}} = K' \left( \mathbb{E} \langle \tilde{W}^\dagger \epsilon_1^\infty, t^\infty \rangle^2 \right)^{\frac{1}{2}} \\ &= K' \left( \mathbb{E} \langle \tilde{\epsilon}_1^\infty, t^\infty \rangle^2 \right)^{\frac{1}{2}} = K' \langle C_{\tilde{\epsilon}} t^\infty, t^\infty \rangle^{\frac{1}{2}}, \end{aligned}$$

where  $C_{\tilde{\epsilon}}$  is the covariance operator of  $\tilde{\epsilon}_1^\infty$ . Taking  $t^\infty = (t_1, \dots, t_p, 0, \dots)^\top \in \ell^2$  and plugging it into the above equation give us

$$\|\langle \tilde{\epsilon}_1, t \rangle\|_{\psi_1} = \|\langle \tilde{\epsilon}_1^\infty, t^\infty \rangle\|_{\psi_1} \leq K' \left( \mathbb{E} \langle \tilde{\epsilon}_1^\infty, t^\infty \rangle^2 \right)^{\frac{1}{2}} = K' \left( \mathbb{E} \langle \tilde{\epsilon}_1, t \rangle^2 \right)^{\frac{1}{2}}.$$

Finally, from (S2), for  $\tilde{\epsilon}_1 = \tilde{\Sigma}^{-\frac{1}{2}} \tilde{\epsilon}_1$ , we deduce that

$$\begin{aligned} \sup_{\|t\|_2=1} \|\langle \tilde{\epsilon}_1, t \rangle\|_{\psi_1} &= \sup_{\|t\|_2=1} \|\langle \tilde{\Sigma}^{-\frac{1}{2}} \tilde{\epsilon}_1, t \rangle\|_{\psi_1} = \sup_{\|t\|_2=1} \|\langle \tilde{\epsilon}_1, \tilde{\Sigma}^{-\frac{1}{2}} t \rangle\|_{\psi_1} \\ &\leq \sup_{\|t\|_2=1} K' \left( \mathbb{E} \langle \tilde{\epsilon}_1, \tilde{\Sigma}^{-\frac{1}{2}} t \rangle^2 \right)^{\frac{1}{2}} = \sup_{\|t\|_2=1} K' \left( \mathbb{E} [t^\top \tilde{\Sigma}^{-\frac{1}{2}} \tilde{\epsilon}_1 \tilde{\epsilon}_1^\top \tilde{\Sigma}^{-\frac{1}{2}} t] \right)^{\frac{1}{2}} \\ &= \sup_{\|t\|_2=1} K' \|t\|_2 = K'. \end{aligned}$$

This shows that  $\tilde{\epsilon}_1$  is a sub-exponential random vector.  $\square$

Below we show that, if  $\Sigma$  shares the desired variance decay condition and the correlation structure,  $\tilde{\Sigma}$  would also satisfy the variance decay condition (Condition (i) of Assumption 2.2) in [Lopes et al. \(2020\)](#) and the correlation structure condition (Equation (3.2)) in [Lopes and Yao \(2022\)](#). Here, we focus on the case that  $d_{\mathcal{X}} = d_{\mathcal{Y}} = \infty$ .

**Proposition S2.2.** *Suppose Assumptions 3.1-3.3 hold, and the variance sequence  $\{\tilde{\sigma}_j^2\}_{j=1}^p$  and the correlation matrix  $\tilde{R}$  of  $\tilde{V}_1$  are induced by  $(\tilde{\phi}, \tilde{\psi}) \in \mathcal{F}_p$ .*

- (i) *The parameters  $\tilde{\sigma}_1, \dots, \tilde{\sigma}_p$  are positive, and there are positive constant  $c_o > 0$ , not depending on  $n$  or  $(\tilde{\phi}, \tilde{\psi})$ , such that*

$$\tilde{\sigma}_{(j)} \geq c_o j^{-\tilde{\alpha}/2} \quad \text{for all } j = 1, \dots, k_n$$

*and  $\{\tilde{\sigma}_{(j)}\}_{j=k_n+1}^p$  is summable in a form similar to (S4), which also gives*

$$\sum_{j=k_n+1}^p \tilde{\sigma}_{(j)} \leq c_o k_n^{-\tilde{\alpha}/2}, \tag{S3}$$

*with  $\tilde{\alpha} = \min\{\underline{\alpha}, \underline{\alpha}_0\}$  and  $\underline{\alpha}_0 = \min\{\alpha_0, \alpha_\star\}$ , where  $\alpha_\star$  is defined in the proof below.*

(ii) Given any constant  $\delta \in (0, 1/2)$ , there is a constant  $c_0 \in (0, 1)$ , not depending on  $n$  or  $(\tilde{\phi}, \tilde{\psi})$ , such that

$$\|\tilde{R}(k_n)\|_F^2 \leq c_0 k_n^{2-\delta}.$$

*Proof.* Part (i). From Lemma S5.3,  $\tilde{\sigma}_j = \sqrt{\tilde{\Sigma}_{jj}} \asymp \sqrt{\Sigma_{jj} + a_n + b_n} > 0$  with  $\Sigma_{jj} = \sigma_j^2$  satisfying the variance decay condition according to Lemma S2.3. To show the variance decay condition for  $\tilde{\sigma}_{(j)}$ , the first step is to show that  $\tilde{\sigma}_{(j)}$  is lower bounded for  $j = 1, \dots, k_n$ , and the second step is to show that  $\tilde{\sigma}_{(j)}$  is upper bounded for  $j = k_n + 1, \dots, p$ .

Consider the case  $j = 1, \dots, k_n$  first. It is clear  $a_n \lesssim k_n^{-\bar{\alpha}}$  by its definition and  $b_n = \max\{p_1^{1-\alpha_1}, p_2^{1-\alpha_2}\} \leq k_n^{-\bar{\alpha}}$  by Assumption 3.3. Therefore,  $\sigma_{(j)}^2 \gtrsim a_n$  with the decreasingly ordered entries  $\sigma_{(1)}^2 \geq \dots \geq \sigma_{(k_n)}^2$ . Moreover,  $\sigma_{(j)}^2 \gtrsim j^{-\bar{\alpha}} \gtrsim k_n^{-\bar{\alpha}} \gtrsim b_n$  with sufficiently large  $n$ . Consequently, we have  $\tilde{\sigma}_{(j)} \geq c_0 j^{-\bar{\alpha}/2}$  for  $j = 1, \dots, k_n$  and sufficiently large  $n$ .

For the case  $j = k_n + 1, \dots, p$ , first note that under our assumptions, we can choose a constant  $\alpha_\star > 0$  such that  $b_n \leq p^{-\alpha_\star}$ . For example, by Assumption 3.3, if  $p_1 > p_2$  and  $p_1 = Cp_2$  for some constant  $C > 1$ , then we can take any  $\alpha_\star < \frac{\alpha-1}{C_0+1}$  with  $C_0 > 1$  being a constant such that  $\log_{p_2} C + 1 \leq C_0$ . Along with  $a_n \lesssim p^{-\alpha_0}$ , we have  $\tilde{\sigma}_{(j)} \lesssim \max\{\sigma_{(j)}, j^{-\underline{\alpha}_0/2}\}$  with  $\underline{\alpha}_0 = \min\{\alpha_0, \alpha_\star\}$  for  $j = k_n + 1, \dots, p$  and sufficiently large  $n$ . By Lemma S2.3,  $\{\sigma_{(j)}\}_{j=k_n+1}^p$  is summable. Note  $\{j^{-\underline{\alpha}_0/2}\}$  also shares the similar summation form of (S4). Therefore,  $\tilde{\sigma}_{(j)}$  is also summable and has the form of (S4) since  $\max\{\sigma_{(j)}, j^{-\underline{\alpha}_0/2}\} \leq \sigma_{(j)} + j^{-\underline{\alpha}_0/2}$ . This leads to (S3).

Part (ii). It can be seen that

$$\tilde{R}_{i,j} = \frac{\tilde{\Sigma}_{ij}}{\sqrt{\tilde{\Sigma}_{ii}}\sqrt{\tilde{\Sigma}_{jj}}} \asymp \frac{\Sigma_{ij} + a_n + b_n}{\sqrt{\Sigma_{ii} + a_n + b_n}\sqrt{\Sigma_{jj} + a_n + b_n}} \asymp \frac{\Sigma_{ij} + a_n + b_n}{\sqrt{\Sigma_{ii}\Sigma_{jj} + a_n + b_n}} \asymp \frac{\Sigma_{ij}}{\sqrt{\Sigma_{ii}}\sqrt{\Sigma_{jj}}} + a_n + b_n = R_{i,j} + a_n + b_n.$$

We claim that the indices of the  $k_n$  largest variances among  $\{\tilde{\sigma}_j\}_{j=1}^p$  would appear in  $\{(1)_o, \dots, (m_n)_o\}$  with  $\sigma_{(j)_o}$  referring to the decreasingly ordered entries of  $\{\sigma_j\}_{j=1}^p$  and  $m_n$  defined in (ii) of Assumption 3.2. This is because we must have  $\tilde{\sigma}_{(j)_o} \lesssim k_n^{-\bar{\alpha}/2}$  for  $j = m_n, \dots, p$ . Otherwise, with the fact that  $|a_n| \lesssim k_n^{-\bar{\alpha}}$  and  $|b_n| \lesssim k_n^{-\bar{\alpha}}$ ,

$$\begin{aligned} \sum_{j=k_n+1}^{m_n} \tilde{\sigma}_{(j)_o} &\gtrsim \sum_{j=k_n+1}^{m_n} \sigma_{(j)_o} - (m_n - k_n)(a_n + b_n) \\ &\gtrsim k_n^{-\bar{\alpha}/2}(m_n - k_n) - (m_n - k_n)k_n^{-\bar{\alpha}} \\ &\asymp k_n^{-\bar{\alpha}/2}(m_n - k_n) \asymp k_n^{-\bar{\alpha}/2+\delta_0} \gtrsim k_n^{-\bar{\alpha}/2}, \end{aligned}$$

contradicting to (S3). Therefore,

$$\begin{aligned} \|\tilde{R}(k_n)\|_F^2 &\lesssim \sup_{R^\circ \in \mathcal{R}(k_n, m_n)} \|R^\circ\|_F^2 + k_n^2 a_n + k_n^2 b_n \\ &\lesssim k_n^{2-\delta} + k_n^2 (k_n^{\bar{\alpha}} p^{\alpha_0})^{-1} + k_n^2 k_n^{-\delta} \asymp k_n^{2-\delta}, \end{aligned}$$

where we use (ii) of Assumption 3.2 and the fact  $b_n \lesssim k_n^{-\bar{\alpha}} \lesssim k_n^{-\delta}$  in the second inequality.  $\square$

Let  $\sigma_{(j)}$  be the decreasingly ordered entries in the sequence  $\{\sigma_j\}$  of the standard deviation of  $V_1$ . The next proposition shows that the sequence  $\{\sigma_j\}$  exhibits a decay pattern.

**Lemma S2.3.** *Given any constant  $\delta \in (0, 1/2)$ , under Assumption 3.2, for  $j = 1, \dots, k_n$ , we have*

$$\sigma_{(j)} \geq c'_0 j^{-\frac{\bar{\alpha}}{2}},$$

for  $\bar{\alpha} = \max\{\alpha_1, \alpha_2\}$ ,  $c'_0 > 0$  and  $k_n$  defined right before the Assumption 3.2. Moreover, for  $\underline{\alpha} = \min\{\alpha_1, \alpha_2\}$ ,  $\tau \in [0, 1)$ ,  $\underline{\beta}_n = \underline{\alpha}(1 - \tau)$  and  $q = \max\{\frac{2}{\underline{\beta}_n}, \log(n), 3\}$ , we have

$$\sum_{j=k_n+1}^p \sigma_{(j)}^{q(1-\tau)} \leq C_0 \frac{k_n^{-q\underline{\beta}_n+1}}{q\underline{\beta}_n-1}, \quad (\text{S4})$$

for some  $C_0 > 0$ , which also gives  $\sigma_{(j)} \lesssim k_n^{-\underline{\alpha}/2}$  for  $j \geq k_n + 1$ .

*Proof.* From Lemma S5.1,  $\Sigma$  is given by

$$\Sigma_{rj} = \begin{cases} (\sum_{l \neq r_1} b_{lr_2}^2 \lambda_l + \tilde{\kappa}_{r_2}) \lambda_{r_1} + b_{r_1 r_2}^2 (\mathbb{E}[(\eta_{1r_1}^X)^4] - 1) \lambda_{r_1}^2 & j_1 = r_1, j_2 = r_2, (r = j), \\ b_{r_1 r_2} b_{r_1 j_2} (\mathbb{E}[(\eta_{1r_1}^X)^4] - 2) \lambda_{r_1}^2 & j_1 = r_1, j_2 \neq r_2, \\ b_{r_1 r_2} b_{j_1 j_2} \lambda_{r_1} \lambda_{j_1} & \text{o.w.} \end{cases}$$

for  $r = p_1(r_2 - 1) + r_1$ ,  $r_1 = 1, \dots, p_1$ ,  $r_2 = 1, \dots, p_2$  and  $j = p_1(j_2 - 1) + j_1$ ,  $j_1 = 1, \dots, p_1$ ,  $j_2 = 1, \dots, p_2$ .

For  $\delta \in (0, 1/2)$ , define  $a = 4 \vee (3\underline{\alpha}(1 - \tau))$  and

$$k_{1,n} = \lceil n^{\frac{\delta}{2a}} \wedge p_1 \rceil, \quad k_{2,n} = \lceil n^{\frac{\delta}{2a}} \wedge p_2 \rceil.$$

Let  $J_{1,n} = \{1, \dots, k_{1,n}\}$ ,  $J_{2,n} = \{1, \dots, k_{2,n}\}$ ,  $J_n = J_{1,n} \times J_{2,n}$  and  $J_n^c = \{1, \dots, p_1\} \times \{1, \dots, p_2\} \setminus J_n$ . Clearly, there is a one-one map between  $\{1, \dots, k_n\}$  with  $k_n = k_{1,n} k_{2,n}$  and  $J_n$ . For  $V_i$ , the order of the variance of the  $j$ th component of  $V_i$  is

$$\sigma_j^2 \asymp \lambda_{j_1} \rho_{j_2}, \quad j = p_1(j_2 - 1) + j_1,$$

due to the condition (11) and Lemma S5.2. Recall  $\lambda_{j_1} \asymp j_1^{-\alpha_1}$ ,  $\rho_{j_2} \asymp j_2^{-\alpha_2}$ . It is seen that for each  $(j_1, j_2) \in J_n$ , there are constants  $c_0, c'_0 \in (0, 1)$ , such that

$$\sigma_j \geq \sqrt{c'_0 \lambda_{j_1} \rho_{j_2}} \geq \sqrt{c_0 j_1^{-\alpha_1} j_2^{-\alpha_2}} \geq \sqrt{c_0 (j_1 j_2)^{-\bar{\alpha}}} \geq \sqrt{c_0 (p_1(j_2 - 1) + j_1)^{-\bar{\alpha}}} = \sqrt{c_0} j^{-\frac{\bar{\alpha}}{2}}.$$

Therefore,

$$\sigma_{(j)} \geq \sigma_j \geq \sqrt{c_0} j^{-\frac{\bar{\alpha}}{2}}.$$

This proves the first statement of the proposition.

Note that for any index set  $I \subset \{1, \dots, p\}$  with  $|I| = p - k_n$ , where  $|I|$  is the cardinality of the set  $I$ , we have

$$\sum_{j=k_n+1}^p \sigma_{(j)} \leq \sum_{j \in I} \sigma_j.$$

Therefore, since  $|J_n^c| = p - |J_n| = p - k_n$ , we further have

$$\begin{aligned} \sum_{j=k_n+1}^p \sigma_{(j)}^{q(1-\tau)} &\leq \sum_{\substack{(j_1, j_2) \in J_n^c \\ j=p_1(j_2-1)+j_1}} \sigma_j^{q(1-\tau)} \\ &= \sum_{j_1 \in J_{1,n}^c} \sum_{j_2=1}^{p_2} \sigma_j^{q(1-\tau)} + \sum_{j_2 \in J_{2,n}^c} \sum_{j_1 \in J_{1,n}} \sigma_j^{q(1-\tau)} \\ &\leq \sum_{j_1 \in J_{1,n}^c} \sum_{j_2=1}^{p_2} C \lambda_{j_1}^{q(1-\tau)} \rho_{j_2}^{q(1-\tau)} + \sum_{j_2 \in J_{2,n}^c} \sum_{j_1=1}^{p_1} C \rho_{j_2}^{q(1-\tau)} \lambda_{j_1}^{q(1-\tau)} \\ &\leq C \left( \sum_{j_1 \in J_{1,n}^c} \lambda_{j_1}^{q(1-\tau)} \sum_{j_2=1}^{p_2} \rho_{j_2}^{q(1-\tau)} + C \sum_{j_2 \in J_{2,n}^c} \rho_{j_2}^{q(1-\tau)} \sum_{j_1=1}^{p_1} \lambda_{j_1}^{q(1-\tau)} \right) \\ &\leq C_1 \left( \sum_{j_1 \in J_{1,n}^c} \lambda_{j_1}^{q(1-\tau)} + \sum_{j_2 \in J_{2,n}^c} \rho_{j_2}^{q(1-\tau)} \right) \\ &\leq C_1 \left( \sum_{j_1=k_{1,n}+1}^{p_1} j_1^{-q\beta_{-n}} + \sum_{j_2=k_{2,n}+1}^{p_2} j_2^{-q\beta_{-n}} \right) \\ &\leq C_1 \left( \int_{k_{1,n}}^{p_1} x^{-q\beta_{-n}} dx + \int_{k_{2,n}}^{p_2} x^{-q\beta_{-n}} dx \right) \\ &\leq C_0 \frac{k_n^{-q\beta_{-n}+1}}{q\beta_{-n}-1}, \end{aligned}$$

where  $C_0 = 2C_2$ . This proves the second statement of the proposition.  $\square$

The next proposition is used in the proof of Theorem 3.7 in Section 3. Recall  $\hat{M} = \hat{M}(\tilde{\phi}, \tilde{\psi})$  and that  $\hat{M}(\tilde{\phi}, \tilde{\psi})$  is defined right before Theorem 3.7.

**Proposition S2.4.** *For any fixed small number  $\delta \in (0, 1/2)$ , if Assumptions 3.1–3.3 hold, then for some constant  $c > 0$ , not depending on  $n$  or  $(\tilde{\psi}, \tilde{\phi})$ , one has*

$$d_K(\mathcal{L}(\hat{M}), \mathcal{L}(\tilde{M})) \leq cn^{-\frac{1}{2}+\delta}.$$

*Proof.* We reuse the proof of Theorem 3.4 in Lin et al. (2022). In that paper, it is mentioned that Assumption 4 therein can be replaced with the condition  $n^{-1/2} \log^3 p \ll 1$  which is satisfied here due to our Assumption 3.3. By examining their proof, we find that it is sufficient to prove Lemma E.7 and Lemma E.8 in Lin et al. (2022) for the sequence  $\{\tilde{V}_i\}_{i=1}^n$  satisfying the assumptions in Lopes et al. (2020). We complete these requirements by Lemmas S2.5 and S2.6 below.  $\square$

For the following two lemmas, we define

$$\hat{M}_d = \max_{j \in \tilde{\mathcal{J}}(d)} \tilde{S}_{n,j} / \hat{\sigma}_j^\tau, \quad (\text{S5})$$

where for any  $d \in \{1, \dots, p\}$ ,  $\tilde{\mathcal{J}}(d)$  denotes a set of indices corresponding to the  $d$  largest values among the standard deviations  $\tilde{\sigma}_1, \dots, \tilde{\sigma}_p$  of the elements in  $\tilde{V}_1$ , i.e.  $\{\tilde{\sigma}_{(1)}, \dots, \tilde{\sigma}_{(p)}\} = \{\tilde{\sigma}_j : j \in \tilde{\mathcal{J}}(d)\}$ .

**Lemma S2.5.** *Under the conditions of Theorem 3.7, for some constant  $c > 0$ , not depending on  $n$  or  $(\tilde{\psi}, \tilde{\phi})$ , we have*

$$\mathbb{P}\left(|\hat{M}_{k_n} - \tilde{M}_{k_n}| > r_n\right) \leq cn^{-1},$$

where  $\hat{M}_{k_n}$  is defined according to (S5) and  $r_n = cn^{-1/2} \log^{5/2} n$ .

*Proof.* Note that Lemma E.4 and Lemma E.3 in Lin et al. (2022), which are the key ingredients for proving Lemma E.7 in Lin et al. (2022), can be replaced by Lemma D.6 and Lemma D.4 in Lopes et al. (2020). The proof is then identical to that for Lemma E.7 in Lin et al. (2022).  $\square$

The next lemma is in analogy to Lemma E.8 in Lin et al. (2022) and can be established also by a similar argument that leads to Lemma E.8 in Lin et al. (2022); we thus omit the proof.

**Lemma S2.6.** *Under Assumptions 3.1 and 3.3, for any number  $\kappa \geq 1$ , there are positive constants  $c$  and  $c_\kappa$ , not depending on  $n$  or  $(\tilde{\psi}, \tilde{\phi})$ , such that the event*

$$\max_{1 \leq j \leq p} \left| \frac{\hat{\sigma}_j^2}{\tilde{\sigma}_j^2} - 1 \right| \leq c_\kappa (\log n + \log^3 p) n^{-\frac{1}{2}}$$

holds with probability at least  $1 - cn^{-\kappa}$ .

### S3 Proof of Theorem 3.6

*Proof.* As in Lopes et al. (2020), we consider the following decomposition

$$\sup_{(\tilde{\phi}, \tilde{\psi}) \in \mathcal{F}_p} d_K(\mathcal{L}(\check{M}_p(\tilde{\phi}, \tilde{\psi})), \mathcal{L}(M_p^*(\tilde{\phi}, \tilde{\psi})|\mathcal{D})) \leq \sup_{(\tilde{\phi}, \tilde{\psi}) \in \mathcal{F}_p} \text{I}'_n + \sup_{(\tilde{\phi}, \tilde{\psi}) \in \mathcal{F}_p} \text{II}'_n(\mathcal{D}) + \sup_{(\tilde{\phi}, \tilde{\psi}) \in \mathcal{F}_p} \text{III}'_n(\mathcal{D}),$$

where

$$\begin{aligned} \text{I}'_n &= d_K(\mathcal{L}(\check{M}_p(\tilde{\phi}, \tilde{\psi})), \mathcal{L}(\check{M}_{k_n}(\tilde{\phi}, \tilde{\psi}))), \\ \text{II}'_n(\mathcal{D}) &= d_K(\mathcal{L}(\check{M}_{k_n}(\tilde{\phi}, \tilde{\psi})), \mathcal{L}(M_{k_n}^*(\tilde{\phi}, \tilde{\psi})|\mathcal{D})), \\ \text{III}'_n(\mathcal{D}) &= d_K(\mathcal{L}(M_{k_n}^*(\tilde{\phi}, \tilde{\psi})|\mathcal{D}), \mathcal{L}(M_p^*(\tilde{\phi}, \tilde{\psi})|\mathcal{D})). \end{aligned}$$

Like in the proof of Section S2, the term  $\sup_{(\tilde{\phi}, \tilde{\psi}) \in \mathcal{F}_p} \text{I}'_n$  is bounded by the rate  $n^{-1/2+\delta}$ . It is then sufficient to show that  $\sup_{(\tilde{\phi}, \tilde{\psi}) \in \mathcal{F}_p} \text{II}'_n(\mathcal{D})$  and  $\sup_{(\tilde{\phi}, \tilde{\psi}) \in \mathcal{F}_p} \text{III}'_n(\mathcal{D})$  can be bounded by the rate  $n^{-1/2+\delta}$  with probability at least  $1 - cn^{-1}$  for some constant  $c > 0$ .

For  $\sup_{(\tilde{\phi}, \tilde{\psi}) \in \mathcal{F}_p} \text{III}'_n(\mathcal{D})$ , given any number  $t'_{1,n} \leq t'_{2,n}$ , we have the decomposition

$$\sup_{(\tilde{\phi}, \tilde{\psi}) \in \mathcal{F}_p} \text{III}'_n(\mathcal{D}) \leq \sup_{(\tilde{\phi}, \tilde{\psi}) \in \mathcal{F}_p} \mathbb{P}(A'(t'_{2,n})|\mathcal{D}) + \sup_{(\tilde{\phi}, \tilde{\psi}) \in \mathcal{F}_p} \mathbb{P}(B'(t'_{1,n})|\mathcal{D}),$$

where  $t'_{1,n}$  and  $t'_{2,n}$  are defined as in Section 5.1 of Lopes and Yao (2022), and for any  $t \in \mathbb{R}$ ,

$$A'(t) = \left\{ \max_{j \in \mathcal{J}_{k_n}(\tilde{\phi}, \tilde{\psi})} S_{n,j}^*(\tilde{\phi}, \tilde{\psi}) / \hat{\sigma}_j^\tau(\tilde{\phi}, \tilde{\psi}) \leq t \right\} \quad \text{and} \quad B'(t) = \left\{ \max_{j \in \mathcal{J}_{k_n}^c(\tilde{\phi}, \tilde{\psi})} S_{n,j}^*(\tilde{\phi}, \tilde{\psi}) / \hat{\sigma}_j^\tau(\tilde{\phi}, \tilde{\psi}) > t \right\}.$$

On the one hand,

$$\mathbb{P}(A'(t'_{2,n})|\mathcal{D}) \leq \mathbb{P}\left( \max_{j \in \mathcal{J}_{\ell_n}(\tilde{\phi}, \tilde{\psi})} \tilde{S}_{n,j}(\tilde{\phi}, \tilde{\psi}) / \hat{\sigma}_j^\tau(\tilde{\phi}, \tilde{\psi}) \leq t'_{2,n} \right) + \sup_{(\tilde{\phi}, \tilde{\psi}) \in \mathcal{F}_p} \text{II}'_n(\mathcal{D}).$$

The first term is at the rate  $n^{-1/2}$  by the similar arguments to establish the equation (5.12) in Lopes and Yao (2022), and the second term will be handled later. On the other hand, defining  $V^*(\tilde{\phi}, \tilde{\psi}) = \max_{j \in \mathcal{J}_{k_n}^c(\tilde{\phi}, \tilde{\psi})} S_{n,j}^*(\tilde{\phi}, \tilde{\psi}) / \hat{\sigma}_j^\tau(\tilde{\phi}, \tilde{\psi})$ , for  $q \leq \log(n)$  and  $c_n \asymp t'_{1,n}$ , if we can show that

$$\sup_{(\tilde{\phi}, \tilde{\psi}) \in \mathcal{F}_p} (\mathbb{E}[|V^*|^q|\mathcal{D}])^{\frac{1}{q}} \leq c_n, \tag{S6}$$

with high probability, we would have

$$\sup_{(\tilde{\phi}, \tilde{\psi}) \in \mathcal{F}_p} \mathbb{P}(B'(t'_{1,n})|\mathcal{D}) = \sup_{(\tilde{\phi}, \tilde{\psi}) \in \mathcal{F}_p} \mathbb{P}(V^* > t'_{1,n}|\mathcal{D}) = \sup_{(\tilde{\phi}, \tilde{\psi}) \in \mathcal{F}_p} \mathbb{P}(V^* > ec_n|\mathcal{D}) \leq \sup_{(\tilde{\phi}, \tilde{\psi}) \in \mathcal{F}_p} e^{-q} \leq n^{-1}.$$

Hence, if  $\sup_{(\tilde{\phi}, \tilde{\psi}) \in \mathcal{F}_p} \text{II}'_n(\mathcal{D}) \lesssim n^{-1/2+\delta}$  and (S6) hold with high probability, then

$$\sup_{(\tilde{\phi}, \tilde{\psi}) \in \mathcal{F}_p} \text{III}'_n(\mathcal{D}) \leq O(n^{-\frac{1}{2}}) + O(n^{-\frac{1}{2}+\delta}) + O(n^{-1}) \asymp O(n^{-\frac{1}{2}+\delta}),$$

also holds with high probability. The inequality (S6) is established by Lemma S3.1 below, and we now focus on  $\sup_{(\tilde{\phi}, \tilde{\psi}) \in \mathcal{F}_p} \text{II}'_n(\mathcal{D}) \lesssim n^{-1/2+\delta}$ .

Consider the triangle inequality

$$\sup_{(\tilde{\phi}, \tilde{\psi}) \in \mathcal{F}_p} \text{II}'_n(\mathcal{D}) \leq \sup_{(\tilde{\phi}, \tilde{\psi}) \in \mathcal{F}_p} d_K(\mathcal{L}(\check{M}_{k_n}(\tilde{\phi}, \tilde{\psi})), \mathcal{L}(\check{M}_{k_n}^*(\tilde{\phi}, \tilde{\psi})|\mathcal{D})) + \sup_{(\tilde{\phi}, \tilde{\psi}) \in \mathcal{F}_p} d_K(\mathcal{L}(\check{M}_{k_n}^*(\tilde{\phi}, \tilde{\psi})), \mathcal{L}(M_{k_n}^*(\tilde{\phi}, \tilde{\psi})|\mathcal{D})),$$

where  $\check{M}_{k_n}^*(\tilde{\phi}, \tilde{\psi}) = \max_{j \in \mathcal{J}_{k_n}(\tilde{\phi}, \tilde{\psi})} S_{n,j}^*(\tilde{\phi}, \tilde{\psi}) / \sigma_j^\tau(\tilde{\phi}, \tilde{\psi})$ . For the first term, one can show, as similar discussions

in [Lopes et al. \(2020\)](#), given  $\epsilon = cn^{-1/2}k_n \log(n)$ , with high probability,

$$\sup_{(\tilde{\phi}, \tilde{\psi}) \in \mathcal{F}_p} d_K(\mathcal{L}(\check{M}_{k_n}(\tilde{\phi}, \tilde{\psi})), \mathcal{L}(\check{M}_{k_n}^*(\tilde{\phi}, \tilde{\psi})|\mathcal{D})) \leq Ck_n^{-\frac{1}{2}}\epsilon \asymp O(n^{-\frac{1}{2}+\delta}), \quad (\text{S7})$$

by Lemma [S3.2](#), the uniform version of Lemma D.5 in [Lopes et al. \(2020\)](#). The second term can be further decomposed into

$$\begin{aligned} & \sup_{(\tilde{\phi}, \tilde{\psi}) \in \mathcal{F}_p} d_K(\mathcal{L}(\check{M}_{k_n}^*(\tilde{\phi}, \tilde{\psi})), \mathcal{L}(M_{k_n}^*(\tilde{\phi}, \tilde{\psi})|\mathcal{D})) \\ & \leq \sup_{(\tilde{\phi}, \tilde{\psi}) \in \mathcal{F}_p} \sup_{t \in \mathbb{R}} \mathbb{P}(|M_{k_n}^*(\tilde{\phi}, \tilde{\psi}) - t| \leq r_n | \mathcal{D}) + \sup_{(\tilde{\phi}, \tilde{\psi}) \in \mathcal{F}_p} \mathbb{P}(|M_{k_n}^*(\tilde{\phi}, \tilde{\psi}) - \check{M}_{k_n}^*(\tilde{\phi}, \tilde{\psi})| > r_n | \mathcal{D}). \end{aligned}$$

The second term in the above inequality without the sup quantifier has been analyzed in [Lopes et al. \(2020\)](#) based on Lemma D.8 in that paper, which in turn essentially depends on Lemma D.2 in the same paper. Our Lemma [S3.1](#) ensures that the above uniform version also holds. For the first term, the key is to analyze

$$\inf_{(\tilde{\phi}, \tilde{\psi}) \in \mathcal{F}_p} \min_{j \in \mathcal{J}_{k_n}(\tilde{\phi}, \tilde{\psi})} \hat{\sigma}_j^{1-\tau},$$

which is handled in Lemma [S3.3](#). With this, the anti-concentration inequality for a Gaussian vector (Nazarov's inequality) can be used to bound  $\sup_{(\tilde{\phi}, \tilde{\psi}) \in \mathcal{F}_p} \sup_{t \in \mathbb{R}} \mathbb{P}(|M_{k_n}^*(\tilde{\phi}, \tilde{\psi}) - t| \leq r_n | \mathcal{D})$ . Along with the above two bounds, with high probability, we have

$$\sup_{(\tilde{\phi}, \tilde{\psi}) \in \mathcal{F}_p} d_K(\mathcal{L}(\check{M}_{k_n}^*(\tilde{\phi}, \tilde{\psi})), \mathcal{L}(M_{k_n}^*(\tilde{\phi}, \tilde{\psi})|\mathcal{D})) \lesssim O(n^{-\frac{1}{2}+\delta}). \quad (\text{S8})$$

Combining [\(S7\)](#) and [\(S8\)](#) yields

$$\sup_{(\tilde{\phi}, \tilde{\psi}) \in \mathcal{F}_p} \Pi'_n(\mathcal{D}) \lesssim O(n^{-\frac{1}{2}+\delta}),$$

with high probability, which completes the proof.  $\square$

**Lemma S3.1.** *Given any number  $\delta \in (0, 1/2)$ , define the parameter  $\beta_n^0 = \alpha_0(1-\tau)$  and assume the conditions of Theorem [3.6](#) hold. Let  $q = \max\{2/\beta_n^0, \log(n), 3\}$  and  $s = q(1-\tau)$ , and consider the random variables  $\hat{\mathbf{s}}$  and  $\hat{\mathbf{t}}$  defined by*

$$\hat{\mathbf{s}}(\tilde{\phi}, \tilde{\psi}) = \left( \sum_{j \in \mathcal{J}_{k_n}^c(\tilde{\phi}, \tilde{\psi})} \hat{\sigma}_j^s(\tilde{\phi}, \tilde{\psi}) \right)^{\frac{1}{s}} \quad \text{and} \quad \hat{\mathbf{t}}(\tilde{\phi}, \tilde{\psi}) = \left( \sum_{j \in \mathcal{J}_{k_n}(\tilde{\phi}, \tilde{\psi})} \hat{\sigma}_j^s(\tilde{\phi}, \tilde{\psi}) \right)^{\frac{1}{s}}.$$

*Then, there is a constant  $c > 0$ , not depending on  $n$  or  $(\tilde{\phi}, \tilde{\psi})$ , such that*

$$\mathbb{P} \left( \sup_{(\tilde{\phi}, \tilde{\psi}) \in \mathcal{F}_p} \hat{\mathbf{s}}(\tilde{\phi}, \tilde{\psi}) \geq \frac{c\sqrt{q}}{(q\beta_n^0 - 1)^{1/s}} \cdot k_n^{-\alpha_0+1/s} \right) \leq cn^{-1}, \quad (\text{S9})$$

and

$$\mathbb{P}\left(\sup_{(\tilde{\phi}, \tilde{\psi}) \in \mathcal{F}_p} \hat{\mathbf{t}}(\tilde{\phi}, \tilde{\psi}) \geq \frac{c\sqrt{q}}{(q\beta_n^0 - 1)^{1/s}}\right) \leq cn^{-1}. \quad (\text{S10})$$

*Proof.* In the following, we assume the variance sequence  $\{\sigma_j\}_{j=1}^p$  of the population version test sequence  $V_1$  is arranged in a decreasing order without loss of generality.

By Markov's inequality,

$$\mathbb{P}\left(\sup_{(\tilde{\phi}, \tilde{\psi}) \in \mathcal{F}_p} \hat{\mathbf{s}}(\tilde{\phi}, \tilde{\psi}) \geq e \left\| \sup_{(\tilde{\phi}, \tilde{\psi}) \in \mathcal{F}_p} \hat{\mathbf{s}}(\tilde{\phi}, \tilde{\psi}) \right\|_q\right) \leq e^{-q}.$$

It suffices to bound  $\left\| \sup_{(\tilde{\phi}, \tilde{\psi}) \in \mathcal{F}_p} \hat{\mathbf{s}}(\tilde{\phi}, \tilde{\psi}) \right\|_q$  (and similarly for  $\sup_{(\tilde{\phi}, \tilde{\psi}) \in \mathcal{F}_p} \hat{\mathbf{t}}(\tilde{\phi}, \tilde{\psi})$ ). By calculation, we have

$$\begin{aligned} \left\| \sup_{(\tilde{\phi}, \tilde{\psi}) \in \mathcal{F}_p} \hat{\mathbf{s}}(\tilde{\phi}, \tilde{\psi}) \right\|_q &= \left( \mathbb{E} \left| \sup_{(\tilde{\phi}, \tilde{\psi}) \in \mathcal{F}_p} \left( \sum_{j \in \mathcal{J}_{k_n}^c(\tilde{\phi}, \tilde{\psi})} \hat{\sigma}_j^s(\tilde{\phi}, \tilde{\psi}) \right) \right|^{1/s} \right)^{1/q} \\ &= \left( \mathbb{E} \left| \left( \sup_{(\tilde{\phi}, \tilde{\psi}) \in \mathcal{F}_p} \sum_{j \in \mathcal{J}_{k_n}^c(\tilde{\phi}, \tilde{\psi})} \hat{\sigma}_j^s(\tilde{\phi}, \tilde{\psi}) \right) \right|^{1/s} \right)^{1/q} \\ &\leq \left( \mathbb{E} \left( \sum_{j=k_n+1}^p \left( \sup_{(\tilde{\phi}, \tilde{\psi}) \in \mathcal{F}_p} \hat{\sigma}_{(j)}(\tilde{\phi}, \tilde{\psi}) \right)^s \right)^{q/s} \right)^{1/q} \\ &= \left\| \sum_{j=k_n+1}^p \hat{\sigma}_j^s \right\|_{q/s}^{1/s} \leq \left( \sum_{j=k_n+1}^p \left\| \hat{\sigma}_j^s \right\|_{q/s} \right)^{1/s} = \left( \sum_{j=k_n+1}^p \left\| \hat{\sigma}_j \right\|_q^s \right)^{1/s}, \end{aligned} \quad (\text{S11})$$

where  $\hat{\sigma}_j = \sup_{(\tilde{\phi}, \tilde{\psi}) \in \mathcal{F}_p} \hat{\sigma}_{(j)}(\tilde{\phi}, \tilde{\psi})$ . Note  $(j)$  may be different for different  $(\tilde{\phi}, \tilde{\psi})$ . We are finding a bound for

$$\left\| \hat{\sigma}_j \right\|_q = \left( \mathbb{E} \left( \sup_{(\tilde{\phi}, \tilde{\psi}) \in \mathcal{F}_p} \hat{\sigma}_{(j)}^2(\tilde{\phi}, \tilde{\psi}) \right)^{q/2} \right)^{1/q}.$$

Since there is an orthogonal matrix  $\tilde{U} \in \mathbb{R}^{p \times p}$  such that  $\tilde{V}_i = \tilde{U}^\top V_i$  with  $\tilde{u}_j \in \mathbb{R}^p$  being the  $j$ th column of  $\tilde{U}$ , one has

$$\begin{aligned} \hat{\sigma}_j^2 &= \frac{1}{n} \sum_{i=1}^n (\tilde{V}_{ij} - \bar{\tilde{V}}_j)^2 = \frac{1}{n} \sum_{i=1}^n ((V_i - \bar{V})^\top \tilde{u}_j)^2 \\ &= \frac{1}{n} \sum_{i=1}^n \left[ (V_{ij} - \bar{V}_j) + (\tilde{u}_{jj} - 1)(V_{ij} - \bar{V}_j) + \sum_{k \neq j} \tilde{u}_{jk}(V_{ik} - \bar{V}_k) \right]^2 \\ &= \frac{1}{n} \sum_{i=1}^n (V_{ij} - \bar{V}_j)^2 + \frac{1}{n} \sum_{i=1}^n (b_j, V_i - \bar{V})^2 + \frac{2}{n} \sum_{i=1}^n (V_{ij} - \bar{V}_j) \langle b_j, V_i - \bar{V} \rangle \\ &\leq \frac{2}{n} \sum_{i=1}^n (V_{ij} - \bar{V}_j)^2 + \frac{2}{n} \sum_{i=1}^n \langle b_j, V_i - \bar{V} \rangle^2 = 2\hat{\sigma}_j^2 + \frac{2}{n} \sum_{i=1}^n \langle b_j, V_i - \bar{V} \rangle^2, \end{aligned}$$

where  $b_j \in \mathbb{R}^p$  is the vector defined by  $b_{jj} = \tilde{u}_{jj} - 1$  and  $b_{jk} = \tilde{u}_{jk}$  with  $k \neq j$ . Noting  $|b_{jk}| \lesssim a_n$  for  $j = 1, \dots, p$  by the construction of  $\mathcal{F}_p$ , one further has

$$\sup_{(\tilde{\phi}, \tilde{\psi}) \in \mathcal{F}_p} \hat{\sigma}_j^2 \leq 2\hat{\sigma}_j^2 + \frac{2}{n} \sum_{i=1}^n \sup_{b \in \mathcal{B}} \langle b, V_i - \bar{V} \rangle^2, \quad (\text{S12})$$

where  $\mathcal{B} = \{b \in \mathbb{R}^p \mid \|b\|_\infty \leq c_0 a_n \text{ and } \|b\|_2 \leq r_0 \text{ for some constants } c_0, r_0 > 0\}$  is the intersection of  $\ell_2$ -ball with radius  $r_0$  and the  $\ell_\infty$ -ball with radius  $c_0 a_n$  in  $\mathbb{R}^p$ .

For the term  $\hat{\sigma}_j^2$  in (S12), according to Lemma D.1 in Lopes et al. (2020),

$$\|\hat{\sigma}_j\|_q \leq c \cdot \sigma_j \cdot \sqrt{q} \quad (\text{S13})$$

holds for some constant  $c > 0$ . For the other term, by Hölder's inequality, we first have

$$\sup_{b \in \mathcal{B}} \langle b, V_i - \bar{V} \rangle^2 \leq \sup_{b \in \mathcal{B}} \|b\|_\infty^2 \|V_i - \bar{V}\|_1^2 \lesssim a_n^2 \|V_i - \bar{V}\|_1^2 = a_n^2 T_i^2,$$

where  $T_i \triangleq \|V_i - \bar{V}\|_1$ . Together with the fact  $\|V_{ij} - \bar{V}_j\|_{\psi_2} \leq C_0$  from Assumption 3.1, we conclude

$$\|T_i^2\|_{\psi_1} = \|T_i\|_{\psi_2}^2 \leq \left( \sum_{j=1}^p \|V_{ij} - \bar{V}_j\|_{\psi_2} \right)^2 \leq p^2 C_0^2.$$

In other words,  $T_i^2 = \|V_i - \bar{V}\|_1^2$  is sub-exponential. Therefore, by the general Bernstein's inequality for sub-exponential random variables, there is a constant  $c > 0$ , for every  $t \geq 0$ , such that

$$\mathbb{P} \left( n^{-1} \sum_{i=1}^n (T_i^2 - \mathbb{E}T_i^2) \geq t \right) \leq 2 \exp \left\{ -c \min \left( \frac{t^2}{p^4 C_0^4}, \frac{t}{p^2 C_0^2} \right) n \right\}. \quad (\text{S14})$$

Taking  $t = k_n^{\bar{\alpha}}$  and if  $\mathbb{E}T_i^2$  is bounded by a constant, by Assumption 3.3, we can assert that  $n^{-1} \sum_{i=1}^n (T_i^2 - \mathbb{E}T_i^2)$  is upper bounded by  $k_n^{\bar{\alpha}}$  with probability at least  $1 - cn^{-1}$  for sufficiently large  $n$ .

Now we verify that  $\mathbb{E}T_i^2$  is bounded. First,

$$\begin{aligned} \mathbb{E}T_i^2 &= \mathbb{E}\|V_i - \bar{V}\|_1^2 \\ &= \mathbb{E} \left[ \sum_{j=1}^p |V_{ij} - \bar{V}_j|^2 + \sum_{1 \leq k \neq j \leq p} |V_{ij} - \bar{V}_j| |V_{ik} - \bar{V}_k| \right] \\ &= \sum_{j=1}^p \mathbb{E}(V_{ij} - \bar{V}_j)^2 + \sum_{1 \leq k \neq j \leq p} \mathbb{E}[|V_{ij} - \bar{V}_j| |V_{ik} - \bar{V}_k|] \\ &\leq \sum_{j=1}^p \mathbb{E}(V_{ij} - \bar{V}_j)^2 + \sum_{1 \leq k \neq j \leq p} \sqrt{\mathbb{E}(V_{ij} - \bar{V}_j)^2} \sqrt{\mathbb{E}(V_{ik} - \bar{V}_k)^2} \\ &\leq \sum_{j=1}^p \mathbb{E}(V_{ij} - \bar{V}_j)^2 + \left( \sum_{j=1}^p \sqrt{\mathbb{E}(V_{ij} - \bar{V}_j)^2} \right) \left( \sum_{k=1}^p \sqrt{\mathbb{E}(V_{ik} - \bar{V}_k)^2} \right) \end{aligned}$$

$$= \sum_{j=1}^p \mathbb{E} (V_{ij} - \bar{V}_j)^2 + \left( \sum_{j=1}^p \sqrt{\mathbb{E} (V_{ij} - \bar{V}_j)^2} \right)^2.$$

In addition, for  $\mathbb{E} (V_{ij} - \bar{V}_j)^2$  with  $j = p_1(j_2 - 1) + j_1$ , we have

$$\begin{aligned} \mathbb{E} (V_{ij} - \bar{V}_j)^2 &= \mathbb{E} (V_{ij}^2 + \bar{V}_j^2 - 2V_{ij}\bar{V}_j) \\ &= \mathbb{E} V_{ij}^2 + \mathbb{E} \left( \frac{1}{n} \sum_{k=1}^n V_{kj} \right)^2 - 2\mathbb{E} \left( \frac{1}{n} \sum_{k=1}^n V_{kj} V_{ij} \right) \\ &= \mathbb{E} V_{ij}^2 + \frac{1}{n} \mathbb{E} V_{ij}^2 + \frac{n-1}{n} \nu_j^2 - \frac{2}{n} (\mathbb{E} V_{ij}^2 + (n-1) \nu_j^2) \\ &= \frac{n-1}{n} (\mathbb{E} V_{ij}^2 - \nu_j^2) \\ &= \frac{n-1}{n} \Sigma_{jj} \\ &= \frac{n-1}{n} \left[ \left( \sum_{l \neq j_1} b_{lj_2}^2 \lambda_l + \tilde{\kappa}_{j_2} \right) \lambda_{j_1} + b_{j_1 j_2}^2 (\mathbb{E}[(\eta_{1j_1}^X)^4] - 1) \lambda_{j_1}^2 \right] \\ &\asymp \lambda_{j_1} \rho_{j_2} \asymp j_1^{-\alpha_1} j_2^{-\alpha_2}, \end{aligned}$$

where  $\nu = \mathbb{E}[V_i]$  and  $\Sigma$  is the covariance matrix of  $V_i$ . By Assumption 3.2, we then conclude that  $\mathbb{E} T_i^2 < \infty$ .

Note that  $n^{-1} \sum_{i=1}^n T_i^2$  is also bounded with high probability according to (S14). Moreover,

$$\sup_{b \in \mathcal{B}} \langle b, V_i - \bar{V} \rangle^2 \lesssim a_n^2 k_n^{2\bar{\alpha}} = p^{-2\alpha_0} < j^{-\alpha_0} \quad (\text{S15})$$

holds with high probability. With (S12), combining (S13) and (S15), for  $j = 1, \dots, p$ , we have

$$\|\hat{\sigma}_j\|_q = \left\| \sup_{(\tilde{\phi}, \tilde{\psi}) \in \mathcal{F}_p} \hat{\sigma}_j(\tilde{\phi}, \tilde{\psi}) \right\|_q \lesssim 2\|\hat{\sigma}_j^2\| + 2j^{-\alpha_0} \leq c\sqrt{q} \max\{\sigma_j, j^{-\alpha_0}\}.$$

By the summation in Lemma S2.3 and the decay pattern of  $\{j^{-\alpha_0}\}$  in the view of (S11), we have

$$\left\| \sup_{(\tilde{\phi}, \tilde{\psi}) \in \mathcal{F}_p} \hat{\mathbf{s}}(\tilde{\phi}, \tilde{\psi}) \right\|_q \lesssim \sqrt{q} \cdot \frac{k_n^{-\alpha_0+1/s}}{(s\alpha_0-1)^{1/s}}$$

with probability  $1 - cn^{-1}$ . Moreover, the fact that  $s\alpha_0 = q\beta_n^0 > 1$  ensures (S9) to hold. Similar argument can be conducted for  $\sup_{(\tilde{\phi}, \tilde{\psi}) \in \mathcal{F}_p} \hat{\mathbf{t}}$ , which ensures (S10) to hold.  $\square$

**Lemma S3.2.** *Let random vectors  $\varepsilon_1(\tilde{\phi}, \tilde{\psi}), \dots, \varepsilon_n(\tilde{\phi}, \tilde{\psi}) \in \mathbb{R}^p$  be as in (S2) for  $(\tilde{\phi}, \tilde{\psi}) \in \mathcal{F}_p$ , and let  $Q(\tilde{\phi}, \tilde{\psi}) \in \mathbb{R}^{p \times \tilde{r}}$  be a deterministic matrix having orthonormal columns with  $\tilde{r} = r(\tilde{\phi}, \tilde{\psi}) \leq k_n$ . Lastly, let*

$$E_n(\tilde{\phi}, \tilde{\psi}) = \frac{1}{n} \sum_{i=1}^n (\varepsilon_i(\tilde{\phi}, \tilde{\psi}) - \bar{\varepsilon}(\tilde{\phi}, \tilde{\psi})) (\varepsilon_i(\tilde{\phi}, \tilde{\psi}) - \bar{\varepsilon}(\tilde{\phi}, \tilde{\psi}))^\top,$$

where  $\bar{\varepsilon}(\tilde{\phi}, \tilde{\psi}) = \frac{1}{n} \sum_{i=1}^n \varepsilon_i(\tilde{\phi}, \tilde{\psi})$ . Then, there is a constant  $c > 0$ , not depending on  $n$  or  $(\tilde{\phi}, \tilde{\psi})$ , such that the event

$$\sup_{(\tilde{\phi}, \tilde{\psi}) \in \mathcal{F}_p} \|Q^\top(\tilde{\phi}, \tilde{\psi})E_n(\tilde{\phi}, \tilde{\psi})Q(\tilde{\phi}, \tilde{\psi}) - I_{\tilde{r}}\|_{\text{op}} \leq \frac{c \log(n)k_n}{\sqrt{n}},$$

holds with probability at least  $1 - cn^{-1}$ .

*Proof.* Noting that  $\tilde{E}_n = \tilde{U}^\top E_n \tilde{U}$  for some unitary matrix  $\tilde{U}$ , we have  $\tilde{r} = r$  for any  $(\tilde{\phi}, \tilde{\psi}) \in \mathcal{F}_p$ . For  $\epsilon \in (0, 1/2)$ , let  $\mathcal{N}$  be an  $\epsilon$ -net (with respect to the  $\ell_2$ -norm) for the unit  $\ell_2$ -sphere in  $\mathbb{R}^r$ . Consider the inequality

$$\|\tilde{Q}^\top \tilde{E}_n \tilde{Q} - I_{\tilde{r}}\|_{\text{op}} \leq \frac{1}{1 - 2\epsilon} \cdot \max_{u \in \mathcal{N}} |u^\top (\tilde{Q}^\top \tilde{E}_n \tilde{Q} - I_r) u|,$$

which holds with probability 1. Taking the supremum, we then have

$$\sup_{(\tilde{\phi}, \tilde{\psi}) \in \mathcal{F}_p} \|\tilde{Q}^\top \tilde{E}_n \tilde{Q} - I_{\tilde{r}}\|_{\text{op}} \leq \frac{1}{1 - 2\epsilon} \cdot \sup_{(\tilde{\phi}, \tilde{\psi}) \in \mathcal{F}_p} \max_{u \in \mathcal{N}} |u^\top (\tilde{Q}^\top \tilde{U}^\top E_n \tilde{U} \tilde{Q} - I_r) u|,$$

with probability 1. Let  $\tilde{P} = \tilde{U} \tilde{Q} \in \mathbb{R}^{p \times r}$  be a deterministic matrix having orthonormal columns. Note that

$$\sup_{(\tilde{\phi}, \tilde{\psi}) \in \mathcal{F}_p} \max_{u \in \mathcal{N}} |u^\top (\tilde{Q}^\top \tilde{U}^\top E_n \tilde{U} \tilde{Q} - I_r) u| = \max_{\tilde{u} \in \tilde{\mathcal{N}}} |\tilde{u}^\top (E_n - I_p) \tilde{u}|,$$

where  $\tilde{u} = \tilde{P}u$ , and  $\tilde{\mathcal{N}}$  is an  $\epsilon$ -net that spans an  $r$ -dimensional subspace of  $\mathbb{R}^p$ . According to the result of Example 27.1 in [Shalev-Shwartz and Ben-David \(2014\)](#) (or Lemma 4.1 in [Pollard \(1990\)](#)),  $\tilde{\mathcal{N}}$  can be chosen such that its cardinality satisfies  $\text{card}(\tilde{\mathcal{N}}) \leq (2\sqrt{r}/\epsilon)^r$ . The rest of the proof is similar to the arguments for Lemma D.5 in [Lopes et al. \(2020\)](#) and thus omitted.  $\square$

**Lemma S3.3.** Suppose the conditions of Theorem 3.6 hold and define the parameter  $\bar{\beta}_n = \bar{\alpha}(1 - \tau)$ . Then, there is a constant  $c > 0$ , not depending on  $n$  or  $(\tilde{\phi}, \tilde{\psi})$ , such that the event

$$\inf_{(\tilde{\phi}, \tilde{\psi}) \in \mathcal{F}_p} \min_{j \in \mathcal{J}_{k_n}(\tilde{\phi}, \tilde{\psi})} \hat{\sigma}_j^{1-\tau} \geq ck_n^{-\bar{\beta}_n/2},$$

holds with probability at least  $1 - cn^{-1}$ .

*Proof.* As in Lemma S3.1, we assume the variance sequence  $\{\sigma_j\}_{j=1}^p$  of the population version test sequence  $V_1$  is arranged in a decreasing order without loss of generality.

Since

$$\inf_{(\tilde{\phi}, \tilde{\psi}) \in \mathcal{F}_p} \min_{j \in \mathcal{J}_{k_n}(\tilde{\phi}, \tilde{\psi})} \hat{\sigma}_j^{1-\tau} \geq \min_{1, \dots, k_n} \inf_{(\tilde{\phi}, \tilde{\psi}) \in \mathcal{F}_p} \hat{\sigma}_{(j)}^{1-\tau}, \quad (\text{S16})$$

we focus on the infimum part first. In the proof of Lemma S3.1, we have shown

$$\hat{\sigma}_j^2 = \hat{\sigma}_j^2 + \frac{1}{n} \sum_{i=1}^n \langle b_j, V_i - \bar{V} \rangle^2 + \frac{2}{n} \sum_{i=1}^n (V_{ij} - \bar{V}_j) \langle b_j, V_i - \bar{V} \rangle \geq \hat{\sigma}_j^2 + \frac{2}{n} \sum_{i=1}^n (V_{ij} - \bar{V}_j) \langle b_j, V_i - \bar{V} \rangle,$$

where  $b_j \in \mathbb{R}^p$  is the vector defined by  $b_{jj} = \tilde{u}_{jj} - 1$  and  $b_{jk} = \tilde{u}_{jk}$  with  $k \neq j$ . Again, we have  $|b_{jk}| \lesssim a_n$  for  $j = 1, \dots, p$ . Therefore,

$$\inf_{(\tilde{\phi}, \tilde{\psi}) \in \mathcal{F}_p} \hat{\sigma}_j^2 \geq \hat{\sigma}_j^2 + \frac{2}{n} \sum_{i=1}^n (V_{ij} - \bar{V}_j) \inf_{b_j \in \mathcal{B}} \langle b_j, V_i - \bar{V} \rangle, \quad (\text{S17})$$

where  $\mathcal{B}$  is defined in Lemma S3.1.

Next, we shall show that for  $j = 1, \dots, k_n$ ,  $\inf_{(\tilde{\phi}, \tilde{\psi}) \in \mathcal{F}_p} \hat{\sigma}_j^2 \gtrsim k_n^{-\bar{\beta}_n/2}$  with high probability. A direct consequence is

$$\min_{1, \dots, k_n} \inf_{(\tilde{\phi}, \tilde{\psi}) \in \mathcal{F}_p} \hat{\sigma}_{(j)}^{1-\tau} \gtrsim k_n^{-\bar{\beta}_n/2},$$

which completes the proof with the help of (S16).

For the first term in (S17), according to Lemma D.6 in Lopes et al. (2020) and the variance decay condition in Lemma S2.3,

$$\hat{\sigma}_j^2 \geq ck_n^{-\bar{\alpha}} \quad (\text{S18})$$

holds with probability at least  $1 - cn^{-1}$  for some constant  $c > 0$ .

For the second term in (S17), in order to bound it from below, observing  $\inf_{b_j \in \mathcal{B}} \langle b_j, V_i - \bar{V} \rangle \geq -\sup_{b_j \in \mathcal{B}} |\langle b_j, V_i - \bar{V} \rangle|$ , we turn to bound

$$\frac{2}{n} \sum_{i=1}^n |V_{ij} - \bar{V}_j| \sup_{b_j \in \mathcal{B}} |\langle b_j, V_i - \bar{V} \rangle|$$

from above first. By Hölder's inequality, this term can be upper bounded by

$$\begin{aligned} \frac{2}{n} \sum_{i=1}^n |V_{ij} - \bar{V}_j| \sup_{b_j \in \mathcal{B}} |\langle b_j, V_i - \bar{V} \rangle| &\leq \frac{2}{n} \sum_{i=1}^n \sup_{b_j \in \mathcal{B}} \|b_j\|_\infty |V_{ij} - \bar{V}_j| \|V_i - \bar{V}\|_1 \\ &\lesssim a_n \frac{2}{n} \sum_{i=1}^n |V_{ij} - \bar{V}_j| \|V_i - \bar{V}\|_1 \\ &= a_n \frac{2}{n} \sum_{i=1}^n \left( \sum_{k=1}^p |V_{ik} - \bar{V}_k| |V_{ij} - \bar{V}_j| \right). \end{aligned}$$

Let  $T_i \triangleq \sum_{k=1}^p |V_{ik} - \bar{V}_k| |V_{ij} - \bar{V}_j|$ . Since  $\|V_{ik} - \bar{V}_k\|_{\psi_2} \leq C_0$  for some constant  $C_0 > 0$  and  $k = 1, \dots, p$ , we have

$$\|T_i\|_{\psi_1} \leq \sum_{k=1}^p \|(V_{ik} - \bar{V}_k)(V_{ij} - \bar{V}_j)\|_{\psi_1} \leq \sum_{k=1}^p \|(V_{ik} - \bar{V}_k)\|_{\psi_2} \|(V_{ij} - \bar{V}_j)\|_{\psi_2} \leq pC_0^2.$$

Therefore, by the general Bernstein's inequality for sub-exponential random variables, there is a constant  $c > 0$ , for every  $t \geq 0$ , such that

$$\mathbb{P} \left( \frac{1}{n} \sum_{i=1}^n (T_i - \mathbb{E}T_i) \geq t \right) \leq 2 \exp \left\{ -c \min \left( \frac{t^2}{p^2 C_0^4}, \frac{t}{p C_0^2} \right) n \right\}.$$

By the similar arguments in the proof of Lemma S3.1, one can show  $\mathbb{E}T_i$  is bounded. Taking  $t = ck_n^{-\bar{\alpha}-\alpha_0}/a_n \gtrsim 1$ , we have  $\mathbb{P}(n^{-1} \sum_{i=1}^n (T_i - \mathbb{E}T_i) \geq ck_n^{-\bar{\alpha}-\alpha_0}/a_n) \leq cn^{-1}$  under Assumption 3.3. Consequently, there is a

constant  $c > 0$ , such that for large enough  $n$ ,

$$\mathbb{P}\left(\frac{2}{n} \sum_{i=1}^n |V_{ij} - \bar{V}_j| \cdot \inf_{b_j \in \mathcal{B}} |\langle b_j, V_i - \bar{V} \rangle| \geq ck_n^{-\bar{\alpha} - \alpha_0}\right) \leq \mathbb{P}\left(\frac{2}{n} \sum_{i=1}^n |V_{ij} - \bar{V}_j| \sup_{b_j \in \mathcal{B}} |\langle b_j, V_i - \bar{V} \rangle| \geq ck_n^{-\bar{\alpha} - \alpha_0}\right) \leq cn^{-1}, \quad (\text{S19})$$

where  $\bar{\alpha} = \max\{\alpha_1, \alpha_2\} > \alpha_0 > 0$ .

Therefore, combining (S18) and (S19) with (S17), there are constants  $c, c', c_1, c_2 > 0$ , such that

$$\inf_{(\tilde{\phi}, \tilde{\psi}) \in \mathcal{F}_p} \hat{\sigma}_j^2 \geq \hat{\sigma}_j^2 - ck_n^{-\bar{\alpha} - \alpha_0} \geq c_0 k_n^{-\bar{\alpha}} (1 - c_1 k_n^{-\alpha_0}) \geq c' k_n^{-\bar{\alpha}}$$

holds with high probability. Together with (S16), we have

$$\inf_{(\tilde{\phi}, \tilde{\psi}) \in \mathcal{F}_p} \min_{j \in \mathcal{J}_{k_n}(\tilde{\phi}, \tilde{\psi})} \hat{\sigma}_j^{1-\tau} \geq \min_{1, \dots, k_n} \inf_{(\tilde{\phi}, \tilde{\psi}) \in \mathcal{F}_p} \hat{\sigma}_{(j)}^{1-\tau} \geq ck_n^{-\bar{\alpha}(1-\tau)/2} = ck_n^{-\bar{\beta}_n/2},$$

with probability at least  $1 - cn^{-1}$ . □

## S4 Uniform Validity and Consistency of the Proposed Test

### S4.1 Proof of Theorem 3.8

*Proof.* On the one hand, from the fact that  $\sup_{i \in I} |x_i| = \max\{\sup_{i \in I} x_i, -\inf_{i \in I} x_i\}$  for any set  $\{x_i, i \in I\}$  with index set  $I$ , to show  $\sup_{(\tilde{\phi}, \tilde{\psi}) \in \mathcal{F}_p} |\text{SIZE}(\varrho, \tilde{\phi}, \tilde{\psi}) - \varrho| \lesssim n^{-1/2+\delta}$  is equivalent to showing

$$\sup_{(\tilde{\phi}, \tilde{\psi}) \in \mathcal{F}_p} \text{SIZE}(\varrho, \tilde{\phi}, \tilde{\psi}) \leq \varrho + O(n^{-\frac{1}{2}+\delta}) \quad \text{and} \quad \inf_{(\tilde{\phi}, \tilde{\psi}) \in \mathcal{F}_p} \text{SIZE}(\varrho, \tilde{\phi}, \tilde{\psi}) \geq \varrho - O(n^{-\frac{1}{2}+\delta}).$$

On the other hand, by definition, for each  $(\tilde{\phi}, \tilde{\psi}) \in \mathcal{F}_p$ , under null hypothesis  $H_0 = \{\nu = 0\}$ ,

$$\begin{aligned} \text{SIZE}(\varrho, \tilde{\phi}, \tilde{\psi}) &= \mathbb{P}\left(\left\{T_U(\tilde{\phi}, \tilde{\psi}) > \hat{q}_{M(\tilde{\phi}, \tilde{\psi})}(1 - \varrho/2)\right\} \cup \left\{T_L(\tilde{\phi}, \tilde{\psi}) < \hat{q}_{L(\tilde{\phi}, \tilde{\psi})}(\varrho/2)\right\} | H_0\right) \\ &= \mathbb{P}\left(T_U(\tilde{\phi}, \tilde{\psi}) > \hat{q}_{M(\tilde{\phi}, \tilde{\psi})}(1 - \varrho/2) | H_0\right) + \mathbb{P}\left(T_L(\tilde{\phi}, \tilde{\psi}) < \hat{q}_{L(\tilde{\phi}, \tilde{\psi})}(\varrho/2) | H_0\right), \end{aligned}$$

where the second equation is from the fact that  $\hat{q}_{M(\tilde{\phi}, \tilde{\psi})}(1 - \varrho/2) > \hat{q}_{L(\tilde{\phi}, \tilde{\psi})}(\varrho/2)$  for  $\varrho < 1/2$  and  $T_U(\tilde{\phi}, \tilde{\psi}) > T_L(\tilde{\phi}, \tilde{\psi})$ . Consequently, combining the results above, it is sufficient to show

$$\begin{aligned} \sup_{(\tilde{\phi}, \tilde{\psi}) \in \mathcal{F}_p} \mathbb{P}\left(T_U(\tilde{\phi}, \tilde{\psi}) > \hat{q}_{M(\tilde{\phi}, \tilde{\psi})}(1 - \varrho/2) | H_0\right) &\leq \varrho/2 + O(n^{-\frac{1}{2}+\delta}), \\ \sup_{(\tilde{\phi}, \tilde{\psi}) \in \mathcal{F}_p} \mathbb{P}\left(T_L(\tilde{\phi}, \tilde{\psi}) < \hat{q}_{L(\tilde{\phi}, \tilde{\psi})}(\varrho/2) | H_0\right) &\leq \varrho/2 + O(n^{-\frac{1}{2}+\delta}), \end{aligned} \quad (\text{S20})$$

and

$$\begin{aligned} \inf_{(\tilde{\phi}, \tilde{\psi}) \in \mathcal{F}_p} \mathbb{P} \left( T_U(\tilde{\phi}, \tilde{\psi}) > \hat{q}_{M(\tilde{\phi}, \tilde{\psi})}(1 - \varrho/2) | H_0 \right) &\geq \varrho/2 - O(n^{-\frac{1}{2} + \delta}), \\ \inf_{(\tilde{\phi}, \tilde{\psi}) \in \mathcal{F}_p} \mathbb{P} \left( T_L(\tilde{\phi}, \tilde{\psi}) < \hat{q}_{L(\tilde{\phi}, \tilde{\psi})}(\varrho/2) | H_0 \right) &\geq \varrho/2 - O(n^{-\frac{1}{2} + \delta}). \end{aligned} \quad (\text{S21})$$

Below we focus on the results (S20) and (S21) for  $T_U(\tilde{\phi}, \tilde{\psi})$ , and the other two results for  $T_L(\tilde{\phi}, \tilde{\psi})$  can be analyzed in a similar fashion.

Define

$$A = \left\{ \sup_{(\tilde{\phi}, \tilde{\psi}) \in \mathcal{F}_p} d_K \left( \mathcal{L}(\hat{M}(\tilde{\phi}, \tilde{\psi})), \mathcal{L}(M^*(\tilde{\phi}, \tilde{\psi}) | \mathcal{D}) \right) \leq cn^{-\frac{1}{2} + \delta} \right\}.$$

According to the discussion in Section 3, based on Theorem 3.5–3.7, we have  $\mathbb{P}(A) \gtrsim 1 - n^{-1}$ . In addition, by the definition of  $\hat{q}_{M(\tilde{\phi}, \tilde{\psi})}(\cdot)$ , for any  $\rho \in (0, 1/2)$ ,  $\mathbb{P}_{|\mathcal{D}} \left( M^*(\tilde{\phi}, \tilde{\psi}) \leq \hat{q}_{M(\tilde{\phi}, \tilde{\psi})}(\rho) | H_0 \right) = \rho$ , where  $\mathbb{P}_{|\mathcal{D}}$  denotes the probability measure conditional on the data  $\mathcal{D}$ . Thus, conditioning on events  $H_0$  and  $A$ , we have

$$\begin{aligned} &\sup_{(\tilde{\phi}, \tilde{\psi}) \in \mathcal{F}_p} \left| \mathbb{P} \left( \hat{M}(\tilde{\phi}, \tilde{\psi}) \leq \hat{q}_{M(\tilde{\phi}, \tilde{\psi})}(\rho) | H_0, A \right) - \rho \right| \\ &= \sup_{(\tilde{\phi}, \tilde{\psi}) \in \mathcal{F}_p} \left| \mathbb{P} \left( \hat{M}(\tilde{\phi}, \tilde{\psi}) \leq \hat{q}_{M(\tilde{\phi}, \tilde{\psi})}(\rho) | H_0, A \right) - \mathbb{P}_{|\mathcal{D}} \left( M^*(\tilde{\phi}, \tilde{\psi}) \leq \hat{q}_{M(\tilde{\phi}, \tilde{\psi})}(\rho) | H_0, A \right) \right| \\ &\lesssim n^{-\frac{1}{2} + \delta}, \end{aligned}$$

which leads to

$$\sup_{(\tilde{\phi}, \tilde{\psi}) \in \mathcal{F}_p} \mathbb{P} \left( \hat{M}(\tilde{\phi}, \tilde{\psi}) \leq \hat{q}_{M(\tilde{\phi}, \tilde{\psi})}(\rho) | H_0, A \right) \lesssim \rho + n^{-\frac{1}{2} + \delta}, \quad (\text{S22})$$

and

$$\inf_{(\tilde{\phi}, \tilde{\psi}) \in \mathcal{F}_p} \mathbb{P} \left( \hat{M}(\tilde{\phi}, \tilde{\psi}) \leq \hat{q}_{M(\tilde{\phi}, \tilde{\psi})}(\rho) | H_0, A \right) \gtrsim \rho - n^{-\frac{1}{2} + \delta}. \quad (\text{S23})$$

For (S20), by the law of total probability,

$$\begin{aligned} &\sup_{(\tilde{\phi}, \tilde{\psi}) \in \mathcal{F}_p} \mathbb{P} \left( T_U(\tilde{\phi}, \tilde{\psi}) > \hat{q}_{M(\tilde{\phi}, \tilde{\psi})}(1 - \varrho/2) | H_0 \right) \\ &\leq \sup_{(\tilde{\phi}, \tilde{\psi}) \in \mathcal{F}_p} \mathbb{P} \left( T_U(\tilde{\phi}, \tilde{\psi}) > \hat{q}_{M(\tilde{\phi}, \tilde{\psi})}(1 - \varrho/2) | H_0, A \right) \mathbb{P}(A | H_0) + \sup_{(\tilde{\phi}, \tilde{\psi}) \in \mathcal{F}_p} \mathbb{P} \left( T_U(\tilde{\phi}, \tilde{\psi}) > \hat{q}_{M(\tilde{\phi}, \tilde{\psi})}(1 - \varrho/2) | H_0, A^c \right) \mathbb{P}(A^c | H_0) \\ &\leq \sup_{(\tilde{\phi}, \tilde{\psi}) \in \mathcal{F}_p} \mathbb{P} \left( T_U(\tilde{\phi}, \tilde{\psi}) > \hat{q}_{M(\tilde{\phi}, \tilde{\psi})}(1 - \varrho/2) | H_0, A \right) + O(n^{-1}) \\ &= \sup_{(\tilde{\phi}, \tilde{\psi}) \in \mathcal{F}_p} \mathbb{P} \left( \hat{M}(\tilde{\phi}, \tilde{\psi}) > \hat{q}_{M(\tilde{\phi}, \tilde{\psi})}(1 - \varrho/2) | H_0, A \right) + O(n^{-1}) \\ &= 1 - \inf_{(\tilde{\phi}, \tilde{\psi}) \in \mathcal{F}_p} \mathbb{P} \left( \hat{M}(\tilde{\phi}, \tilde{\psi}) \leq \hat{q}_{M(\tilde{\phi}, \tilde{\psi})}(1 - \varrho/2) | H_0, A \right) + O(n^{-1}) \\ &\leq 1 - (1 - \varrho/2) + O(n^{-\frac{1}{2} + \delta}) + O(n^{-1}) \\ &= \varrho/2 + O(n^{-\frac{1}{2} + \delta}), \end{aligned}$$

where the fact that  $\hat{M}(\tilde{\phi}, \tilde{\psi}) = T_U(\tilde{\phi}, \tilde{\psi})$  under  $H_0$  is used in the fourth line, and (S23) is used in the sixth line. Similarly, we establish (S21) by the following derivations:

$$\begin{aligned}
& \inf_{(\tilde{\phi}, \tilde{\psi}) \in \mathcal{F}_p} \mathbb{P} \left( T_U(\tilde{\phi}, \tilde{\psi}) > \hat{q}_{M(\tilde{\phi}, \tilde{\psi})}(1 - \varrho/2) | H_0 \right) \\
& \geq \inf_{(\tilde{\phi}, \tilde{\psi}) \in \mathcal{F}_p} \mathbb{P} \left( T_U(\tilde{\phi}, \tilde{\psi}) > \hat{q}_{M(\tilde{\phi}, \tilde{\psi})}(1 - \varrho/2) | H_0, A \right) \mathbb{P}(A | H_0) + \inf_{(\tilde{\phi}, \tilde{\psi}) \in \mathcal{F}_p} \mathbb{P} \left( T_U(\tilde{\phi}, \tilde{\psi}) > \hat{q}_{M(\tilde{\phi}, \tilde{\psi})}(1 - \varrho/2) | H_0, A^c \right) \mathbb{P}(A^c | H_0) \\
& \geq \inf_{(\tilde{\phi}, \tilde{\psi}) \in \mathcal{F}_p} \mathbb{P} \left( T_U(\tilde{\phi}, \tilde{\psi}) > \hat{q}_{M(\tilde{\phi}, \tilde{\psi})}(1 - \varrho/2) | H_0, A \right) (1 - O(n^{-1})) \\
& \geq \inf_{(\tilde{\phi}, \tilde{\psi}) \in \mathcal{F}_p} \mathbb{P} \left( \hat{M}(\tilde{\phi}, \tilde{\psi}) > \hat{q}_{M(\tilde{\phi}, \tilde{\psi})}(1 - \varrho/2) | H_0, A \right) (1 - O(n^{-1})) \\
& = 1 - \sup_{(\tilde{\phi}, \tilde{\psi}) \in \mathcal{F}_p} \mathbb{P} \left( \hat{M}(\tilde{\phi}, \tilde{\psi}) \leq \hat{q}_{M(\tilde{\phi}, \tilde{\psi})}(1 - \varrho/2) | H_0, A \right) (1 - O(n^{-1})) \\
& \geq 1 - (1 - \varrho/2) - O(n^{-\frac{1}{2} + \delta}) + O(n^{-1}) \\
& = \varrho/2 - O(n^{-\frac{1}{2} + \delta}),
\end{aligned}$$

where (S22) is used in the sixth line. □

## S4.2 Proof of Theorem 3.9

*Proof.* Part 2 is handled in Lemma S4.1, while part 1 can be derived as in the proof of Theorem 3.3 in Lin et al. (2022) by replacing the condition event in that paper to  $E = \{\sup_{(\tilde{\phi}, \tilde{\psi}) \in \mathcal{F}_p} d_K(\mathcal{L}(M(\tilde{\phi}, \tilde{\psi})), \mathcal{L}(M^*(\tilde{\phi}, \tilde{\psi}))) \lesssim n^{-1/2 + \delta}\}$ , which has shown to hold with probability at least  $1 - cn^{-1}$  according to Theorem 3.5 and Theorem 3.6.

Now we analyze the uniform consistency of the proposed test over  $\mathcal{F}_p$ . Given  $(\tilde{\phi}, \tilde{\psi}) \in \mathcal{F}_p$ , since  $\tilde{T}_U \geq \tilde{T}_L$  and  $\hat{q}_{\tilde{M}}(1 - \varrho/2) \geq \hat{q}_{\tilde{L}}(\varrho/2)$  for  $\varrho \in (0, 1/2)$ , the two events

$$\tilde{T}_U > \hat{q}_{\tilde{M}}(1 - \varrho/2) \quad \text{and} \quad \tilde{T}_L < \hat{q}_{\tilde{L}}(\varrho/2),$$

can not hold simultaneously. Below we consider the case  $\hat{q}_{\tilde{M}}(1 - \varrho/2) \geq 0 \geq \hat{q}_{\tilde{L}}(\varrho/2)$  with  $\varrho \in (0, 1/2)$ . Other cases can be analyzed in a similar fashion.

We focus on the power function

$$\mathbb{P} \left( \forall (\tilde{\phi}, \tilde{\psi}) \in \mathcal{F}_p, \{ \tilde{T}_U > \hat{q}_{\tilde{M}}(1 - \varrho/2) \} \cup \{ \tilde{T}_L < \hat{q}_{\tilde{L}}(\varrho/2) \} \middle| \mathcal{A}_n \right), \quad (*)$$

where  $\mathcal{A}_n = \{\nu_0 = \max_{1 \leq j \leq p} |\nu_j(\phi, \psi)| \gtrsim \max\{\sigma_{\max}(\phi, \psi) n^{-1/2} \log^{1/2} n, a_n\}\}$ . Note that the conditional event

$$\max_{1 \leq j \leq p} |\nu_j(\phi, \psi)| \gtrsim \max\{\sigma_{\max}(\phi, \psi) n^{-1/2} \log^{1/2} n, a_n\},$$

can be divided into two parts.

- Positive part: Consider the case  $\mathcal{A}_n = \left\{ \max_{1 \leq j \leq p} \nu_j(\phi, \psi) \geq c \max\{\sigma_{\max}(\phi, \psi) n^{-1/2} \log^{1/2} n, a_n\} \right\}$ . Define the events

$$\begin{aligned}\mathcal{A}_n^1 &= \left\{ \sup_{(\tilde{\phi}, \tilde{\psi}) \in \mathcal{F}_p} |\hat{q}_{\tilde{M}}(\varrho)| \leq c_1 \log^{1/2} n \right\}, \\ \mathcal{A}_n^2 &= \left\{ \sup_{(\tilde{\phi}, \tilde{\psi}) \in \mathcal{F}_p} \frac{\max_{1 \leq j \leq p} \hat{\sigma}_j^2}{\tilde{\sigma}_{\max}^2} < 5 \right\}, \\ \mathcal{A}_n^3 &= \left\{ \sup_{(\tilde{\phi}, \tilde{\psi}) \in \mathcal{F}_p} |\tilde{V}_{\tilde{j}} - \tilde{\nu}_{\tilde{j}}| \leq c_2 a_n \right\},\end{aligned}$$

for some  $\tilde{j} \in \{1, \dots, p\}$  depending on  $(\tilde{\phi}, \tilde{\psi})$  and some constant  $c, c_1, c_2 > 0$ . Then, the power function (\*) can be bounded from below by

$$\begin{aligned} (*) &= \mathbb{P} \left( \bigcap_{(\tilde{\phi}, \tilde{\psi}) \in \mathcal{F}_p} (\{ \tilde{T}_U > \hat{q}_{\tilde{M}}(1 - \varrho/2) \} \cup \{ \tilde{T}_L < \hat{q}_{\tilde{L}}(\varrho/2) \}) \middle| \mathcal{A}_n \right) \\ &\geq \mathbb{P} \left( \bigcap_{(\tilde{\phi}, \tilde{\psi}) \in \mathcal{F}_p} \{ \tilde{T}_U > \hat{q}_{\tilde{M}}(1 - \varrho/2) \} \middle| \mathcal{A}_n \right) \\ &= \mathbb{P} \left( \bigcap_{(\tilde{\phi}, \tilde{\psi}) \in \mathcal{F}_p} \left\{ \frac{\tilde{V}_{\tilde{j}}}{\hat{\sigma}_{\tilde{j}}^\tau / \sqrt{n}} > \hat{q}_{\tilde{M}}(1 - \varrho/2) \right\} \middle| \mathcal{A}_n \right) \\ &\geq \mathbb{P} \left( \inf_{(\tilde{\phi}, \tilde{\psi}) \in \mathcal{F}_p} \frac{\tilde{V}_{\tilde{j}}}{\hat{\sigma}_{\tilde{j}}^\tau / \sqrt{n}} > \sup_{(\tilde{\phi}, \tilde{\psi}) \in \mathcal{F}_p} \hat{q}_{\tilde{M}}(1 - \varrho/2) \middle| \mathcal{A}_n, \mathcal{A}_n^1 \right) \mathbb{P}(\mathcal{A}_n^1 | \mathcal{A}_n) \\ &\geq \mathbb{P} \left( \inf_{(\tilde{\phi}, \tilde{\psi}) \in \mathcal{F}_p} \frac{\tilde{V}_{\tilde{j}}}{\hat{\sigma}_{\tilde{j}}^\tau / \sqrt{n}} > c_1 \log^{1/2} n \middle| \mathcal{A}_n, \mathcal{A}_n^1 \right) \mathbb{P}(\mathcal{A}_n^1 | \mathcal{A}_n) \\ &= \mathbb{P} \left( \inf_{(\tilde{\phi}, \tilde{\psi}) \in \mathcal{F}_p} \frac{\tilde{V}_{\tilde{j}} - \tilde{\nu}_{\tilde{j}} + \tilde{\nu}_{\tilde{j}}}{\hat{\sigma}_{\tilde{j}}^\tau / \sqrt{n}} > c_1 \log^{1/2} n \middle| \mathcal{A}_n, \mathcal{A}_n^1 \right) \mathbb{P}(\mathcal{A}_n^1 | \mathcal{A}_n) \\ &= \mathbb{P} \left( \inf_{(\tilde{\phi}, \tilde{\psi}) \in \mathcal{F}_p} \frac{\tilde{V}_{\tilde{j}} - \tilde{\nu}_{\tilde{j}} + \tilde{\nu}_{\tilde{j}}}{\hat{\sigma}_{\tilde{j}}^\tau / \sqrt{n}} > c_1 \log^{1/2} n \middle| \mathcal{A}_n, \mathcal{A}_n^1, \mathcal{A}_n^3 \right) \mathbb{P}(\mathcal{A}_n^1 | \mathcal{A}_n) \mathbb{P}(\mathcal{A}_n^3 | \mathcal{A}_n, \mathcal{A}_n^1) \\ &\geq \mathbb{P} \left( \inf_{(\tilde{\phi}, \tilde{\psi}) \in \mathcal{F}_p} \frac{\tilde{\nu}_{\tilde{j}} - c_2 a_n}{\hat{\sigma}_{\tilde{j}}^\tau / \sqrt{n}} > c_1 \log^{1/2} n \middle| \mathcal{A}_n, \mathcal{A}_n^1, \mathcal{A}_n^3 \right) \mathbb{P}(\mathcal{A}_n^1 | \mathcal{A}_n) \mathbb{P}(\mathcal{A}_n^3 | \mathcal{A}_n, \mathcal{A}_n^1) \\ &\geq \mathbb{P} \left( \inf_{(\tilde{\phi}, \tilde{\psi}) \in \mathcal{F}_p} \frac{\nu_{\tilde{j}}(\phi, \psi) + c_3 a_n - c_2 a_n}{\hat{\sigma}_{\tilde{j}}^\tau / \sqrt{n}} > c_1 \log^{1/2} n \middle| \mathcal{A}_n, \mathcal{A}_n^1, \mathcal{A}_n^3 \right) \mathbb{P}(\mathcal{A}_n^1 | \mathcal{A}_n) \mathbb{P}(\mathcal{A}_n^3 | \mathcal{A}_n, \mathcal{A}_n^1) \\ &\geq \mathbb{P} \left( \frac{\max_{1 \leq j \leq p} \nu_j(\phi, \psi) + c_4 a_n}{\sup_{(\tilde{\phi}, \tilde{\psi}) \in \mathcal{F}_p} \hat{\sigma}_{\tilde{j}}^\tau / \sqrt{n}} > c_1 \log^{1/2} n \middle| \mathcal{A}_n, \mathcal{A}_n^1, \mathcal{A}_n^3 \right) \mathbb{P}(\mathcal{A}_n^1 | \mathcal{A}_n) \mathbb{P}(\mathcal{A}_n^3 | \mathcal{A}_n, \mathcal{A}_n^1) \\ &\geq \mathbb{P} \left( \frac{\max_{1 \leq j \leq p} \nu_j(\phi, \psi) + c_4 a_n}{\sigma_{\max}(\phi, \psi) / \sqrt{n}} > c_5 \log^{1/2} n \middle| \mathcal{A}_n, \mathcal{A}_n^1, \mathcal{A}_n^2, \mathcal{A}_n^3 \right) \mathbb{P}(\mathcal{A}_n^1 | \mathcal{A}_n) \mathbb{P}(\mathcal{A}_n^3 | \mathcal{A}_n, \mathcal{A}_n^1) \mathbb{P}(\mathcal{A}_n^2 | \mathcal{A}_n, \mathcal{A}_n^1, \mathcal{A}_n^3) \\ &\geq \mathbb{P} \left( \max_{1 \leq j \leq p} \nu_j(\phi, \psi) \geq c \max\{\sigma_{\max}(\phi, \psi) n^{-1/2} \log^{1/2} n, a_n\} \middle| \mathcal{A}_n, \mathcal{A}_n^1, \mathcal{A}_n^2, \mathcal{A}_n^3 \right) \left( 1 - \frac{c'_1}{n} \right) \mathbb{P}(\mathcal{A}_n^3 | \mathcal{A}_n, \mathcal{A}_n^1) \left( 1 - \frac{c'_2}{n} \right) \\ &\rightarrow 1. \end{aligned}$$

Here,  $\tilde{\nu}_j = \nu_j(\phi, \psi) + c_3 a_n$ , with all constants to be positive and  $c_3 > c_2 > 0$ . In addition, we use the fact that  $\frac{\sigma_{\max}(\tilde{\phi}, \tilde{\psi})}{\sigma_{\max}(\phi, \psi)} = O(1)$  as mentioned in Lemma S4.1, and  $\mathbb{P}(\mathcal{A}_n^3 | \mathcal{A}_n, \mathcal{A}_n^1) \rightarrow 1$ , as  $n \rightarrow \infty$ , is from Lemma S4.2.

- The case of  $\min_{1 \leq j \leq p} \nu_j(\tilde{\phi}, \tilde{\psi}) \leq -c\sigma_{\max}(\tilde{\phi}, \tilde{\psi})n^{-1/2} \log^{1/2} n$ : This is similar to the above one, and corresponds to the other part of the critical region, i.e.,  $\{T_L(\tilde{\phi}, \tilde{\psi}) < \hat{q}_{L(\tilde{\phi}, \tilde{\psi})}(\varrho/2)\}$ .

□

**Lemma S4.1.** *Suppose Assumptions 3.1-3.3 hold. Then, for some constant  $c > 0$  not depending on  $n$  or  $(\tilde{\phi}, \tilde{\psi})$ , one has*

$$\mathbb{P}\left(\sup_{(\tilde{\phi}, \tilde{\psi}) \in \mathcal{F}_p} \frac{\max_{1 \leq j \leq p} \hat{\sigma}_j^2(\tilde{\phi}, \tilde{\psi})}{\sigma_{\max}^2(\tilde{\phi}, \tilde{\psi})} < 5\right) \geq 1 - cn^{-1},$$

where  $\sigma_{\max}(\tilde{\phi}, \tilde{\psi}) = \max\{\sigma_j(\tilde{\phi}, \tilde{\psi}) : 1 \leq j \leq p\}$ .

*Proof.* First, note that for any  $(\tilde{\phi}, \tilde{\psi}) \in \mathcal{F}_p$ ,

$$\sigma_{\max}^2(\tilde{\phi}, \tilde{\psi}) = \max_{1 \leq j \leq p} \sigma_j^2(\tilde{\phi}, \tilde{\psi}) = \max_{1 \leq j \leq p} (\sigma_j^2(\phi, \psi) + O(a_n)) = \sigma_{\max}^2(\phi, \psi) + O(a_n),$$

where  $a_n = (k_n^\alpha p^{\alpha_0})^{-1} = o(1)$  is in the definition of  $\mathcal{F}_p$ . Further, by (S12) and (S15), the following inequality holds with probability at least  $1 - c_1 n^{-1}$  for large enough  $n$ ,

$$\sup_{(\tilde{\phi}, \tilde{\psi}) \in \mathcal{F}_p} \max_{1 \leq j \leq p} \hat{\sigma}_j^2(\tilde{\phi}, \tilde{\psi}) \leq 2 \max_{1 \leq j \leq p} \hat{\sigma}_j^2(\phi, \psi) + \frac{2}{n} \sum_{i=1}^n \sup_{b \in \mathcal{B}} \langle b, V_i - \bar{V} \rangle^2 \leq 2 \max_{1 \leq j \leq p} \hat{\sigma}_j^2(\phi, \psi) + Cp^{-2\alpha_0}.$$

With the above results, for large enough  $n$  and constants  $c, c_1, c_2 > 0$ , it can be seen that

$$\begin{aligned} \mathbb{P}\left(\sup_{(\tilde{\phi}, \tilde{\psi}) \in \mathcal{F}_p} \frac{\max_{1 \leq j \leq p} \hat{\sigma}_j^2(\tilde{\phi}, \tilde{\psi})}{\sigma_{\max}^2(\tilde{\phi}, \tilde{\psi})} > 5\right) &\leq \mathbb{P}\left(\sup_{(\tilde{\phi}, \tilde{\psi}) \in \mathcal{F}_p} \max_{1 \leq j \leq p} \hat{\sigma}_j^2(\tilde{\phi}, \tilde{\psi}) > 5 \inf_{(\tilde{\phi}, \tilde{\psi}) \in \mathcal{F}_p} \sigma_{\max}^2(\tilde{\phi}, \tilde{\psi})\right) \\ &\leq \mathbb{P}\left(2 \max_{1 \leq j \leq p} \hat{\sigma}_j^2(\phi, \psi) + Cp^{-2\alpha_0} > 5\sigma_{\max}^2(\phi, \psi) + O(a_n)\right) \left(1 - \frac{c_1}{n}\right) + \frac{c_1}{n} \\ &\leq \mathbb{P}\left(\max_{1 \leq j \leq p} \hat{\sigma}_j^2(\phi, \psi) > \frac{5}{2}\sigma_{\max}^2(\phi, \psi) + O(a_n) - O(p^{-2\alpha_0})\right) \left(1 - \frac{c_1}{n}\right) + \frac{c_1}{n} \\ &\leq \mathbb{P}\left(\max_{1 \leq j \leq p} \hat{\sigma}_j^2(\phi, \psi) > 2\sigma_{\max}^2(\phi, \psi)\right) \left(1 - \frac{c_1}{n}\right) + \frac{c_1}{n} \\ &\leq \frac{c_2}{n} \left(1 - \frac{c_1}{n}\right) + \frac{c_1}{n} \leq \frac{c}{n}. \end{aligned}$$

The second line is due to the law of total probability with the conditional event  $\{\sup_{(\tilde{\phi}, \tilde{\psi}) \in \mathcal{F}_p} \max_{1 \leq j \leq p} \hat{\sigma}_j^2(\tilde{\phi}, \tilde{\psi}) \leq 2 \max_{1 \leq j \leq p} \hat{\sigma}_j^2(\phi, \psi) + Cp^{-2\alpha_0}\}$ . The fourth line is due to the fact  $a_n \lesssim p^{-\alpha_0}$  and Lemma S5.1 so that  $\sigma_{\max}(\phi, \psi) = O(1) \gtrsim O(a_n) - O(p^{-2\alpha_0})$ . Moreover, since we have checked the assumptions needed in Lin et al. (2022) in Section S2 for test sequence induced by  $(\phi, \psi)$ , the last line follows from Theorem 3.3 in Lin et al. (2022). □

**Lemma S4.2.** Under Assumption 3.2 and 3.3, for any  $j = 1, \dots, p$ , there is a constant  $c > 0$  such that

$$\mathbb{P} \left( \sup_{(\tilde{\phi}, \tilde{\psi}) \in \mathcal{F}_p} |\bar{V}_j(\tilde{\phi}, \tilde{\psi}) - \nu_j(\tilde{\phi}, \tilde{\psi})| \leq ca_n \right) \rightarrow 1$$

as  $n \rightarrow \infty$ , where  $a_n$  is from the definition of  $\mathcal{F}_p$ .

*Proof.* Recall  $\bar{V}_j(\tilde{\phi}, \tilde{\psi}) = n^{-1} \sum_{i=1}^n V_{ij}(\tilde{\phi}, \tilde{\psi})$  and  $\mathbb{E}V_{1j}(\tilde{\phi}, \tilde{\psi}) = \nu_j(\tilde{\phi}, \tilde{\psi})$ . For  $(\tilde{\phi}, \tilde{\psi}) \in \mathcal{F}_p$ , since  $\{\tilde{\phi}_1, \tilde{\phi}_2, \dots\}$  and  $\{\tilde{\psi}_1, \tilde{\psi}_2, \dots\}$  are orthonormal bases of  $\mathcal{X}$  and  $\mathcal{Y}$  respectively, there is a fixed unitary infinite matrix  $U(\tilde{\phi}, \tilde{\psi})$  such that  $V_1(\tilde{\phi}, \tilde{\psi}) = U(\tilde{\phi}, \tilde{\psi})^\top V_1(\phi, \psi)$ , leading to  $V_{ij}(\tilde{\phi}, \tilde{\psi}) = \langle U_j(\tilde{\phi}, \tilde{\psi}), V_i(\phi, \psi) \rangle_\infty$  for  $j = 1, \dots, p$ , where  $U_j(\tilde{\phi}, \tilde{\psi})$  is the  $j$ th column of  $U(\tilde{\phi}, \tilde{\psi})$  with unit length and  $\langle \cdot, \cdot \rangle_\infty$  is the canonical inner product on  $\ell^2$ .

Therefore, we have

$$\begin{aligned} \sup_{(\tilde{\phi}, \tilde{\psi}) \in \mathcal{F}_p} |\bar{V}_j(\tilde{\phi}, \tilde{\psi}) - \nu_j(\tilde{\phi}, \tilde{\psi})| &= \sup_{(\tilde{\phi}, \tilde{\psi}) \in \mathcal{F}_p} \left| n^{-1} \sum_{i=1}^n \sum_{k=1}^\infty (U_{jk}(\tilde{\phi}, \tilde{\psi}) V_{ik}(\phi, \psi) - \mathbb{E}[U_{jk}(\tilde{\phi}, \tilde{\psi}) V_{ik}(\phi, \psi)]) \right| \\ &\leq \sup_{(\tilde{\phi}, \tilde{\psi}) \in \mathcal{F}_p} \left| n^{-1} \sum_{i=1}^n \sum_{k=1}^p (U_{jk}(\tilde{\phi}, \tilde{\psi}) V_{ik}(\phi, \psi) - \mathbb{E}[U_{jk}(\tilde{\phi}, \tilde{\psi}) V_{ik}(\phi, \psi)]) \right| \\ &\quad + \sup_{(\tilde{\phi}, \tilde{\psi}) \in \mathcal{F}_p} \left| n^{-1} \sum_{i=1}^n \sum_{k=p+1}^\infty (U_{jk}(\tilde{\phi}, \tilde{\psi}) V_{ik}(\phi, \psi) - \mathbb{E}[U_{jk}(\tilde{\phi}, \tilde{\psi}) V_{ik}(\phi, \psi)]) \right| \\ &\leq \sup_{(\tilde{\phi}, \tilde{\psi}) \in \mathcal{F}_p} \left| n^{-1} \sum_{i=1}^n \sum_{k=1}^p (U_{jk}(\tilde{\phi}, \tilde{\psi}) V_{ik}(\phi, \psi) - \mathbb{E}[U_{jk}(\tilde{\phi}, \tilde{\psi}) V_{ik}(\phi, \psi)]) \right| \\ &\quad + \sup_{(\tilde{\phi}, \tilde{\psi}) \in \mathcal{F}_p} \left| \sum_{k=p+1}^\infty U_{jk}(\tilde{\phi}, \tilde{\psi}) (\bar{V}_k(\phi, \psi) - \mathbb{E}\bar{V}_k(\phi, \psi)) \right| \end{aligned} \quad (\text{S24})$$

where  $U_{jk}(\tilde{\phi}, \tilde{\psi})$  and  $V_{ik}(\phi, \psi)$  are the  $k$ th elements of  $U_j(\tilde{\phi}, \tilde{\psi})$  and  $V_i(\phi, \psi)$  respectively, and  $\bar{V}_k(\phi, \psi) = n^{-1} \sum_{i=1}^n V_{ik}(\phi, \psi)$ .

For the first term on the right-hand side of (S24),

$$\sup_{(\tilde{\phi}, \tilde{\psi}) \in \mathcal{F}_p} \left| n^{-1} \sum_{i=1}^n \sum_{k=1}^p (U_{jk}(\tilde{\phi}, \tilde{\psi}) V_{ik}(\phi, \psi) - \mathbb{E}[U_{jk}(\tilde{\phi}, \tilde{\psi}) V_{ik}(\phi, \psi)]) \right| = \sup_{b \in \mathbb{B}_p} \left| n^{-1} \sum_{i=1}^n \langle b, V_i(\phi, \psi) \rangle - \mathbb{E} \langle b, V(\phi, \psi) \rangle \right|, \quad (\text{S25})$$

where  $V(\phi, \psi)$  is the population version of  $V_i(\phi, \psi)$  and  $\mathbb{B}_p = \{b \in \mathbb{R}^p \mid \|b\|_2 \leq 1\}$  is the  $\ell_2$ -ball with unit length in  $\mathbb{R}^p$ . Denote  $V = V(\phi, \psi)$  and  $V_i = V_i(\phi, \psi)$ . By Markov's inequality, we have

$$\mathbb{P} \left( \sup_{b \in \mathbb{B}_p} \left| n^{-1} \sum_{i=1}^n \langle b, V_i \rangle - \mathbb{E} \langle b, V \rangle \right| \geq t \right) \leq \frac{\mathbb{E} \left[ \sup_{b \in \mathbb{B}_p} \left| n^{-1} \sum_{i=1}^n \langle b, V_i \rangle - \mathbb{E} \langle b, V \rangle \right| \right]}{t}. \quad (\text{S26})$$

We bound the expectation first. Given any  $b \in \mathbb{B}_p$ , write  $V^b = n^{-1} \sum_{i=1}^n \langle b, V_i \rangle - \mathbb{E} \langle b, V \rangle$ . For  $a, b \in \mathbb{B}_p$ , it is seen that

$$\|V^b - V^a\|_{\psi_2} = n^{-1} \left\| \sum_{i=1}^n \Delta_i \right\|_{\psi_2},$$

where  $\Delta_i = \langle b - a, V_i \rangle - \mathbb{E} \langle b - a, V \rangle$  are independent with zero mean. Moreover, by Proposition 2.6.1 in

Vershynin (2018),

$$\|V^b - V^a\|_{\psi_2} \lesssim n^{-1} \left( \sum_{i=1}^n \|\Delta_i\|_{\psi_2}^2 \right)^{1/2}.$$

By Assumption 3.1 and centering of a sub-gaussian random variable, we also have

$$\|\Delta_i\|_{\psi_2} \lesssim \|\langle b - a, V_i \rangle\|_{\psi_2} \lesssim \|b - a\|_2.$$

With the above two inequalities, we conclude that

$$\|V^b - V^a\|_{\psi_2} \lesssim n^{-1} \sqrt{n} \|b - a\|_2 = \frac{1}{\sqrt{n}} \|b - a\|_2.$$

This leads to

$$\begin{aligned} \mathbb{E} \left[ \sup_{b \in \mathbb{B}_p} \left| n^{-1} \sum_{i=1}^n \langle b, V_i \rangle - \mathbb{E} \langle b, V \rangle \right| \right] &= \mathbb{E} \left[ \sup_{b \in \mathbb{B}_p} |V^b| \right] = \mathbb{E} \left[ \sup_{b \in \mathbb{B}_p} |V^b - V^0| \right] \\ &\lesssim \frac{1}{\sqrt{n}} \int_0^2 \sqrt{\log \mathcal{N}(\mathbb{B}_p, \|\cdot\|_2, \varepsilon)} d\varepsilon \\ &\lesssim \frac{1}{\sqrt{n}} \sqrt{p} \int_0^2 \sqrt{\log \left( \frac{1}{\varepsilon} + 1 \right)} d\varepsilon \lesssim \frac{\sqrt{p}}{\sqrt{n}}, \end{aligned}$$

where we apply Dudley's inequality in the second line.

Therefore, from (S26), for a suitable  $t > 0$ ,

$$\mathbb{P} \left( \sup_{b \in \mathbb{B}_p} \left| \frac{1}{n} \sum_{i=1}^n \langle b, V_i \rangle - \mathbb{E} \langle b, V \rangle \right| \geq t \right) \leq \frac{1}{t} \frac{\sqrt{p}}{\sqrt{n}}.$$

Taking  $t = ca_n \gtrsim \sqrt{p/n}$  and plugging it into the above equation, due to (S25), we have

$$\mathbb{P} \left( \sup_{(\tilde{\phi}, \tilde{\psi}) \in \mathcal{F}_p} \left| n^{-1} \sum_{i=1}^n \sum_{k=1}^p (U_{jk}(\tilde{\phi}, \tilde{\psi}) V_{ik}(\phi, \psi) - \mathbb{E}[U_{jk}(\tilde{\phi}, \tilde{\psi}) V_{ik}(\phi, \psi)]) \right| \geq ca_n \right) \leq \frac{1}{ca_n} \sqrt{\frac{p}{n}}. \quad (\text{S27})$$

For the second term on the right-hand side of (S24), by Cauchy-Schwartz inequality,

$$\begin{aligned} \sup_{(\tilde{\phi}, \tilde{\psi}) \in \mathcal{F}_p} \left| \sum_{k=p+1}^{\infty} U_{jk}(\tilde{\phi}, \tilde{\psi}) (\bar{V}_k(\phi, \psi) - \mathbb{E} \bar{V}_k(\phi, \psi)) \right| &\leq \sup_{(\tilde{\phi}, \tilde{\psi}) \in \mathcal{F}_p} \left( \sum_{k=p+1}^{\infty} U_{jk}^2(\tilde{\phi}, \tilde{\psi}) \right)^{1/2} \left( \sum_{k=p+1}^{\infty} (\bar{V}_k(\phi, \psi) - \mathbb{E} \bar{V}_k(\phi, \psi))^2 \right)^{1/2} \\ &\leq \left( \sum_{k=p+1}^{\infty} (\bar{V}_k(\phi, \psi) - \mathbb{E} \bar{V}_k(\phi, \psi))^2 \right)^{1/2}, \end{aligned} \quad (\text{S28})$$

where the second inequality holds since  $U_j(\tilde{\phi}, \tilde{\psi})$  is a vector in  $\ell^2$  with unit length. Denote  $V_{ik} = V_{ik}(\phi, \psi)$

and  $\bar{V} = \bar{V}(\phi, \psi)$  as before, and recall  $\bar{V}_k = n^{-1} \sum_{i=1}^n V_{ik}$ . By Markov's inequality, we have

$$\begin{aligned} \mathbb{P}\left(\sum_{k=p+1}^{\infty} (\bar{V}_k - \mathbb{E}\bar{V}_k)^2 \geq t\right) &\leq \frac{\mathbb{E}\left[\sum_{k=p+1}^{\infty} (\bar{V}_k - \mathbb{E}\bar{V}_k)^2\right]}{t} \\ &= \frac{\sum_{k=p+1}^{\infty} [\mathbb{E}\bar{V}_k^2 - (\mathbb{E}\bar{V}_k)^2]}{t} = \frac{\sum_{k=p+1}^{\infty} [\mathbb{E}V_{1k}^2 - (\mathbb{E}V_{1k})^2]}{nt}. \end{aligned} \quad (\text{S29})$$

For a given  $k \geq p+1$ ,  $V_{1k} = \langle X_1, \phi_{k_1} \rangle_1 \langle Y_1, \psi_{k_2} \rangle_2$  with  $(k_1, k_2) = k$  (see the remark on the general notations about  $(k_1, k_2)$  at the beginning of this Supplementary Material), then by Lemma S5.1, Assumption 3.2-(i) and Lemma S5.2,

$$\begin{aligned} 0 \leq \mathbb{E}V_{1k}^2 - (\mathbb{E}V_{1k})^2 &= \Sigma_{(k_1, k_2)(k_1, k_2)}^{\infty} \\ &= \left( \sum_{l \neq k_1} b_{lk_2}^2 \lambda_l + \tilde{\kappa}_{k_2} \right) \lambda_{k_1} + b_{k_1 k_2}^2 (\mathbb{E}[(\eta_{1k_1}^X)^4] - 1) \lambda_{k_1}^2 \\ &\asymp \rho_{k_2} \lambda_{k_1} + \rho_{k_2} \lambda_{k_1}^2 \end{aligned}$$

Consequently,

$$\begin{aligned} \sum_{k=p+1}^{\infty} [\mathbb{E}V_{1k}^2 - (\mathbb{E}V_{1k})^2] &= \sum_{k_1=p_1+1}^{\infty} \sum_{k_2=p_2+1}^{\infty} (\rho_{k_2} \lambda_{k_1} + \rho_{k_2} \lambda_{k_1}^2) + \sum_{k_1=1}^{p_1} \sum_{k_2=p_2+1}^{\infty} (\rho_{k_2} \lambda_{k_1} + \rho_{k_2} \lambda_{k_1}^2) + \sum_{k_1=p_1+1}^{\infty} \sum_{k_2=1}^{p_2} (\rho_{k_2} \lambda_{k_1} + \rho_{k_2} \lambda_{k_1}^2) \\ &\asymp b_n, \end{aligned} \quad (\text{S30})$$

where  $b_n = \max\{p_1^{1-\alpha_1}, p_2^{1-\alpha_2}\}$ .

Inserting (S30) in (S29) and taking  $t = c^2 a_n^2$  in (S29), we have

$$\mathbb{P}\left(\sum_{k=p+1}^{\infty} (\bar{V}_k - \mathbb{E}\bar{V}_k)^2 \geq c^2 a_n^2\right) \leq \frac{b_n}{n} \frac{c^2}{a_n^2}.$$

By (S28), the above inequality further leads to

$$\mathbb{P}\left(\sup_{(\tilde{\phi}, \tilde{\psi}) \in \mathcal{F}_p} \left| \sum_{k=p+1}^{\infty} U_{jk}(\tilde{\phi}, \tilde{\psi}) (\bar{V}_k(\phi, \psi) - \mathbb{E}\bar{V}_k(\phi, \psi)) \right| \geq ca_n\right) \leq \frac{b_n}{n} \frac{1}{c^2 a_n^2}. \quad (\text{S31})$$

Combing (S24) with (S27) and (S31), one has

$$\begin{aligned} \mathbb{P}\left(\sup_{(\tilde{\phi}, \tilde{\psi}) \in \mathcal{F}_p} |\bar{V}_j(\tilde{\phi}, \tilde{\psi}) - \nu_j(\tilde{\phi}, \tilde{\psi})| \geq ca_n\right) &\leq \mathbb{P}\left(\sup_{(\tilde{\phi}, \tilde{\psi}) \in \mathcal{F}_p} \left| n^{-1} \sum_{i=1}^n \sum_{k=1}^p (U_{jk}(\tilde{\phi}, \tilde{\psi}) V_{ik}(\phi, \psi) - \mathbb{E}[U_{jk}(\tilde{\phi}, \tilde{\psi}) V_{ik}(\phi, \psi)]) \right| \right. \\ &\quad \left. + \sup_{(\tilde{\phi}, \tilde{\psi}) \in \mathcal{F}_p} \left| \sum_{k=p+1}^{\infty} U_{jk}(\tilde{\phi}, \tilde{\psi}) (\bar{V}_k(\phi, \psi) - \mathbb{E}\bar{V}_k(\phi, \psi)) \right| \geq ca_n\right) \\ &\leq \mathbb{P}\left(\sup_{(\tilde{\phi}, \tilde{\psi}) \in \mathcal{F}_p} \left| n^{-1} \sum_{i=1}^n \sum_{k=1}^p (U_{jk}(\tilde{\phi}, \tilde{\psi}) V_{ik}(\phi, \psi) - \mathbb{E}[U_{jk}(\tilde{\phi}, \tilde{\psi}) V_{ik}(\phi, \psi)]) \right| \geq \frac{c}{2} a_n\right) \end{aligned}$$

$$\begin{aligned} & \mathbb{P} \left( \sup_{(\tilde{\phi}, \tilde{\psi}) \in \mathcal{F}_p} \left| \sum_{k=p+1}^{\infty} U_{jk}(\tilde{\phi}, \tilde{\psi}) (\bar{V}_k(\phi, \psi) - \mathbb{E} \bar{V}_k(\phi, \psi)) \right| \geq \frac{c}{2} a_n \right) \\ & \leq \frac{2}{ca_n} \sqrt{\frac{p}{n}} + \frac{b_n}{n} \frac{4}{c^2 a_n^2} \rightarrow 0, \end{aligned}$$

as  $n \rightarrow \infty$ . This completes the proof.  $\square$

## S5 Auxiliary Results

**Lemma S5.1.** *The covariance matrix  $\Sigma^\infty$  of  $V_1^\infty(\phi, \psi)$ , defined right before Assumption 3.1, is given by*

$$\Sigma_{(r_1, r_2)(j_1, j_2)}^\infty = \begin{cases} (\sum_{l \neq r_1} b_{lr_2}^2 \lambda_l + \tilde{\kappa}_{r_2}) \lambda_{r_1} + b_{r_1 r_2}^2 (\mathbb{E}[(\eta_{1r_1}^X)^4] - 1) \lambda_{r_1}^2 & j_1 = r_1, j_2 = r_2, (r = j), \\ b_{r_1 r_2} b_{r_1 j_2} (\mathbb{E}[(\eta_{1r_1}^X)^4] - 2) \lambda_{r_1}^2 & j_1 = r_1, j_2 \neq r_2, \\ b_{r_1 r_2} b_{j_1 j_2} \lambda_{r_1} \lambda_{j_1} & o.w. \end{cases}$$

*Proof.* As an operator from  $\ell^2$  to  $\ell^2$ ,  $\Sigma^\infty$  can be treated as an infinite matrix. We use  $\Sigma_{(r_1, r_2)(j_1, j_2)}^\infty$  to indicate the element of  $\Sigma^\infty$  at the  $(r_1, r_2)$ th row and  $(j_1, j_2)$ th column for  $r_1, r_2, j_1, j_2 \geq 1$ ; see also the remark on the general notations about  $(r_1, r_2)$  and  $(j_1, j_2)$  at the beginning of this Supplementary Material as well as Lemma S5.3. Moreover, by definition,  $\Sigma$ , the covariance matrix of  $V_1(\phi, \psi)$  defined in Section 2, is the leading principal minor of the infinite matrix  $\Sigma^\infty$  of order  $p$ . Thus,  $\Sigma_{rj} = \Sigma_{(r_1, r_2)(j_1, j_2)}^\infty$  for  $r = p_1(r_2 - 1) + r_1$ ,  $j = p_1(j_2 - 1) + j_1$  and  $r_1, j_1 = 1, \dots, p_1$ ,  $r_2, j_2 = 1, \dots, p_2$ .

By definition, for  $r_1, r_2, j_1, j_2 \geq 1$ , we have

$$\Sigma_{(r_1, r_2)(j_1, j_2)}^\infty = \mathbb{E}[(V_{1(r_1, r_2)}^\infty - \nu_{(r_1, r_2)}^\infty)(V_{1(j_1, j_2)}^\infty - \nu_{(j_1, j_2)}^\infty)] = \mathbb{E}[V_{1(r_1, r_2)}^\infty V_{1(j_1, j_2)}^\infty] - \nu_{(r_1, r_2)}^\infty \nu_{(j_1, j_2)}^\infty.$$

Below we calculate  $\nu_{(r_1, r_2)}^\infty \nu_{(j_1, j_2)}^\infty$  and  $\mathbb{E}[V_{1(r_1, r_2)}^\infty V_{1(j_1, j_2)}^\infty]$  separately.

First, for  $\nu^\infty$ , we have

$$\begin{aligned} \nu_{(j_1, j_2)}^\infty &= \mathbb{E}[\langle X_1, \phi_{j_1} \rangle \langle Y_1, \psi_{j_2} \rangle] = \mathbb{E}[\langle X_1, \phi_{j_1} \rangle \langle \beta(X_1) + Z_1, \psi_{j_2} \rangle] \\ &= \mathbb{E}[\langle X_1, \phi_{j_1} \rangle \langle \beta(X_1), \psi_{j_2} \rangle] + \mathbb{E}[\langle X_1, \phi_{j_1} \rangle \langle Z_1, \psi_{j_2} \rangle] \\ &= \sum_{k=1}^{\infty} b_{kj_2} \mathbb{E}[\langle X_1, \phi_{j_1} \rangle \langle X_1, \phi_k \rangle] = b_{j_1 j_2} \lambda_{j_1}. \end{aligned}$$

Therefore,

$$\nu_{(r_1, r_2)}^\infty \nu_{(j_1, j_2)}^\infty = b_{r_1 r_2} b_{j_1 j_2} \lambda_{r_1} \lambda_{j_1}, \quad r_1, r_2, j_1, j_2 \geq 1.$$

Next, we turn to  $\mathbb{E}[V_{1(r_1, r_2)}^\infty V_{1(j_1, j_2)}^\infty]$ . For any  $r_1, r_2, j_1, j_2 \geq 1$ ,

$$\begin{aligned} V_{1(r_1, r_2)}^\infty V_{1(j_1, j_2)}^\infty &= \langle X_1, \phi_{r_1} \rangle \langle Y_1, \psi_{r_2} \rangle \langle X_1, \phi_{j_1} \rangle \langle Y_1, \psi_{j_2} \rangle \\ &= \langle X_1, \phi_{r_1} \rangle \langle \beta(X_1) + Z_1, \psi_{r_2} \rangle \langle X_1, \phi_{j_1} \rangle \langle \beta(X_1) + Z_1, \psi_{j_2} \rangle \end{aligned}$$

$$\begin{aligned}
&= \langle X_1, \phi_{r_1} \rangle \langle X_1, \phi_{j_1} \rangle (\langle \beta(X_1), \psi_{r_2} \rangle + \langle Z_1, \psi_{r_2} \rangle) (\langle \beta(X_1), \psi_{j_2} \rangle + \langle Z_1, \psi_{j_2} \rangle) \\
&= \sqrt{\lambda_{r_1} \lambda_{j_1}} \eta_{r_1}^X \eta_{j_1}^X \left( \sum_{k=1}^{\infty} b_{k,r_2} \sqrt{\lambda_k} \eta_k^X + \langle Z_1, \psi_{r_2} \rangle \right) \left( \sum_{k=1}^{\infty} b_{k,j_2} \sqrt{\lambda_k} \eta_k^X + \langle Z_1, \psi_{j_2} \rangle \right) \\
&= \sum_{k=1}^{\infty} \sum_{l=1}^{\infty} b_{k,r_2} b_{l,j_2} \sqrt{\lambda_k \lambda_l} \eta_k^X \eta_l^X \sqrt{\lambda_{r_1} \lambda_{j_1}} \eta_{r_1}^X \eta_{j_1}^X + \langle Z_1, \psi_{r_2} \rangle \langle Z_1, \psi_{j_2} \rangle \sqrt{\lambda_{r_1} \lambda_{j_1}} \eta_{r_1}^X \eta_{j_1}^X \\
&\quad + \sum_{k=1}^{\infty} b_{k,r_2} \sqrt{\lambda_k} \eta_k^X \langle Z_1, \psi_{j_2} \rangle \sqrt{\lambda_{r_1} \lambda_{j_1}} \eta_{r_1}^X \eta_{j_1}^X + \sum_{k=1}^{\infty} b_{k,j_2} \sqrt{\lambda_k} \eta_k^X \langle Z_1, \psi_{r_2} \rangle \sqrt{\lambda_{r_1} \lambda_{j_1}} \eta_{r_1}^X \eta_{j_1}^X.
\end{aligned}$$

By calculation, one can show that

$$\Sigma_{(r_1, r_2)(j_1, j_2)}^{\infty} = \begin{cases} (\sum_{l \neq r_1} b_{lr_2}^2 \lambda_l + \tilde{\kappa}_{r_2}) \lambda_{r_1} + b_{r_1 r_2}^2 (\mathbb{E}[(\eta_{1r_1}^X)^4] - 1) \lambda_{r_1}^2 & j_1 = r_1, j_2 = r_2, (r = j), \\ (\sum_{l \neq r_1} b_{lr_2} b_{lj_2} \lambda_l + \mathbb{E}[\langle Z_1, \psi_{r_2} \rangle \langle Z_1, \psi_{j_2} \rangle]) \lambda_{r_1} + b_{r_1 r_2} b_{r_1 j_2} (\mathbb{E}[(\eta_{1r_1}^X)^4] - 1) \lambda_{r_1}^2 & j_1 = r_1, j_2 \neq r_2, \\ b_{r_1 r_2} b_{j_1 j_2} \lambda_{r_1} \lambda_{j_1} & \text{o.w.} \end{cases}$$

Observing

$$0 = \mathbb{E} \langle Y, \psi_{r_2} \rangle \langle Y, \psi_{j_2} \rangle = \sum_{l=1}^{\infty} b_{lr_2} b_{lj_2} \lambda_l + \mathbb{E}[\langle Z, \psi_{r_2} \rangle \langle Z, \psi_{j_2} \rangle],$$

we also have

$$\sum_{l \neq r_1} b_{lr_2} b_{lj_2} \lambda_l + \mathbb{E}[\langle Z_1, \psi_{r_2} \rangle \langle Z_1, \psi_{j_2} \rangle] = -b_{r_1 r_2} b_{r_1 j_2} \lambda_{r_1}.$$

This allows us to write  $\Sigma^{\infty}$  as

$$\Sigma_{(r_1, r_2)(j_1, j_2)}^{\infty} = \begin{cases} (\sum_{l \neq r_1} b_{lr_2}^2 \lambda_l + \tilde{\kappa}_{r_2}) \lambda_{r_1} + b_{r_1 r_2}^2 (\mathbb{E}[(\eta_{1r_1}^X)^4] - 1) \lambda_{r_1}^2 & j_1 = r_1, j_2 = r_2, (r = j), \\ b_{r_1 r_2} b_{r_1 j_2} (\mathbb{E}[(\eta_{1r_1}^X)^4] - 2) \lambda_{r_1}^2 & j_1 = r_1, j_2 \neq r_2, \\ b_{r_1 r_2} b_{j_1 j_2} \lambda_{r_1} \lambda_{j_1} & \text{o.w.} \end{cases}$$

□

**Lemma S5.2.** Suppose the triple  $(X, Y, Z)$  follows the model (3). Recall that for  $j_2 \geq 1$ ,  $\tilde{\kappa}_{j_2} = \mathbb{E} \langle Z, \psi_{j_2} \rangle^2$  with  $\psi_{j_2}$  from (S1). Then, under Assumption 3.2(i),  $\{\tilde{\kappa}_{j_2}\}_{j_2=1}^{\infty}$  shares the same decay pattern as  $\{\rho_{j_2}\}_{j_2=1}^{\infty}$ , that is,  $\tilde{\kappa}_{j_2} \asymp \rho_{j_2} \asymp j_2^{-\alpha_2}$  for  $j_2 \geq 1$ .

*Proof.* For  $j_2 \geq 1$ , we observe

$$\begin{aligned}
\rho_{j_2} &= \mathbb{E}[\langle Y_i, \psi_{j_2} \rangle^2] = \mathbb{E}[\langle \beta(X_i) + Z_i, \psi_{j_2} \rangle^2] \\
&= \mathbb{E}[\langle \beta(X_i), \psi_{j_2} \rangle^2] + \mathbb{E}[\langle Z_i, \psi_{j_2} \rangle^2] = \mathbb{E}[(\sum_{k=1}^{\infty} b_{kj_2} \sqrt{\lambda_k} \eta_k^X)^2] + \tilde{\kappa}_{j_2} \\
&= \mathbb{E}[\sum_{k=1}^{\infty} b_{kj_2}^2 \lambda_k (\eta_k^X)^2] + \tilde{\kappa}_{j_2} = \sum_{k=1}^{\infty} b_{kj_2}^2 \lambda_k + \tilde{\kappa}_{j_2},
\end{aligned}$$

where the fifth equality is from the Cauchy product and the uncorrelatedness among  $\eta_k^X$ 's. Therefore, with the condition (11), we have  $\tilde{\kappa}_{j_2} \asymp \rho_{j_2}$  for  $j_2 \geq 1$ . This shows that,  $\{\rho_{j_2}\}_{j_2=1}^{\infty}$  and  $\{\tilde{\kappa}_{j_2}\}_{j_2=1}^{\infty}$  share the same decay pattern. □

Recall  $a_n = (k_n^{\bar{\alpha}} p^{\alpha_0})^{-1}$ . The following lemma states that the covariance matrix  $\tilde{\Sigma}$  of  $\tilde{V}_1$  is close to the covariance matrix  $\Sigma$  of  $V_1$ .

**Lemma S5.3.** *Under Assumptions 3.2 and 3.3, for any  $(\tilde{\phi}, \tilde{\psi}) \in \mathcal{F}_p$ , we have*

$$\|\tilde{\Sigma} - \Sigma\|_{\infty} \lesssim a_n + b_n,$$

with  $a_n = (k_n^{\bar{\alpha}} p^{\alpha_0})^{-1}$  and  $b_n = \max\{p_1^{1-\alpha_1}, p_2^{1-\alpha_2}\}$ . Moreover, if  $d_{\mathcal{X}} < \infty$  and  $d_{\mathcal{Y}} < \infty$ ,  $\|\tilde{\Sigma} - \Sigma\|_{\infty} \lesssim a_n$ .

*Proof.* We suppress  $(\tilde{\phi}, \tilde{\psi})$  from  $W_p(\tilde{\phi}, \tilde{\psi})$  to further simplify notations. Define

$$W_{(r_1, r_2)(j_1, j_2)}^{\infty} = \langle \phi_{r_1}, \tilde{\phi}_{j_1} \rangle \langle \psi_{r_2}, \tilde{\psi}_{j_2} \rangle,$$

for  $r_1, j_1, r_2, j_2 \geq 1$ ; see also the remark on the general notations about  $(r_1, r_2)$  and  $(j_1, j_2)$  at the beginning of this Supplementary Material. Moreover, define  $W_{rj}^{\infty} = W_{(r_1, r_2)(j_1, j_2)}^{\infty}$  for  $r = p_1(r_2 - 1) + r_1$ ,  $j = p_1(j_2 - 1) + j_1$ ,  $r_1, j_1 = 1, \dots, p_1$  and  $r_2, j_2 = 1, \dots, p_2$ . Note  $W_{rj} = W_{rj}^{\infty}$  for  $r, j = 1, \dots, p$ . Also,  $|W_{rj}^{\infty}| \leq 1$  holds trivially.

For  $r = p_1(r_2 - 1) + r_1$  and  $j = p_1(j_2 - 1) + j_1$  with  $r_1, j_1 = 1, \dots, p_1$  and  $r_2, j_2 = 1, \dots, p_2$ ,

$$\begin{aligned} \tilde{\Sigma}_{rj} - \Sigma_{rj} &= \mathbb{E}[\tilde{V}_{1r} \tilde{V}_{1j}] - \Sigma_{rj} \\ &= \mathbb{E}[\langle X_1, \tilde{\phi}_{r_1} \rangle \langle Y_1, \tilde{\psi}_{r_2} \rangle \langle X_1, \tilde{\phi}_{j_1} \rangle \langle Y_1, \tilde{\psi}_{j_2} \rangle] - \Sigma_{rj} \\ &= \sum_{m_1=1}^{\infty} \sum_{m_2=1}^{\infty} \sum_{n_1=1}^{\infty} \sum_{n_2=1}^{\infty} \langle \tilde{\phi}_{r_1}, \phi_{m_1} \rangle \langle \tilde{\psi}_{r_2}, \psi_{m_2} \rangle \langle \tilde{\phi}_{j_1}, \phi_{n_1} \rangle \langle \tilde{\psi}_{j_2}, \psi_{n_2} \rangle \Sigma_{(m_1, m_2)(n_1, n_2)}^{\infty} - \Sigma_{rj} \\ &= \sum_{m_1=1}^{\infty} \sum_{m_2=1}^{\infty} \sum_{n_1=1}^{\infty} \sum_{n_2=1}^{\infty} W_{(r_1, r_2)(m_1, m_2)}^{\infty} W_{(j_1, j_2)(n_1, n_2)}^{\infty} \Sigma_{(m_1, m_2)(n_1, n_2)}^{\infty} - \Sigma_{rj} \\ &= A + A_0 + A_1 + A_2 + A_3 + A_4, \end{aligned}$$

where  $A$  and  $A_k, k = 0, \dots, 4$  are defined as follows. First, we define  $A = W_{rr} W_{jj} \Sigma_{rj} - \Sigma_{rj}$ . Then, we observe that, in the summation, the range of  $m_k, n_k, k = 1, 2$  can be divided into two parts. For  $m_1$  and  $n_1$ , the range is  $I_1 \cup I_1^c$ , where  $I_1 = \{1, \dots, p_1\}$  and  $I_1^c = \{p_1 + 1, \dots, \infty\}$ . For  $m_2$  and  $n_2$ , the range is  $I_2 \cup I_2^c$ , where  $I_2 = \{1, \dots, p_2\}$  and  $I_2^c = \{p_2 + 1, \dots, \infty\}$ . We call  $I_1^c$  and  $I_2^c$  the infinite summation parts. With these notations, we define

$$\begin{aligned} A_0 &= \sum_{\substack{m_k, n_k \in I_k \\ k=1,2}} W_{rm} W_{jn} \Sigma_{mn} - W_{rr} W_{jj} \Sigma_{rj} \\ A_1 &= \sum_{\substack{m_1 \in I_1^c, n_1 \in I_1 \\ m_2, n_2 \in I_2}} W_{(r_1, r_2)(m_1, m_2)}^{\infty} W_{(j_1, j_2)(n_1, n_2)}^{\infty} \Sigma_{(m_1, m_2)(n_1, n_2)}^{\infty} + \sum_{\substack{n_1 \in I_1^c, m_1 \in I_1 \\ m_2, n_2 \in I_2}} W_{(r_1, r_2)(m_1, m_2)}^{\infty} W_{(j_1, j_2)(n_1, n_2)}^{\infty} \Sigma_{(m_1, m_2)(n_1, n_2)}^{\infty} \\ &\quad + \sum_{\substack{m_2 \in I_2^c, n_2 \in I_2 \\ m_1, n_1 \in I_1}} W_{(r_1, r_2)(m_1, m_2)}^{\infty} W_{(j_1, j_2)(n_1, n_2)}^{\infty} \Sigma_{(m_1, m_2)(n_1, n_2)}^{\infty} + \sum_{\substack{n_2 \in I_2^c, m_2 \in I_2 \\ m_1, n_1 \in I_1}} W_{(r_1, r_2)(m_1, m_2)}^{\infty} W_{(j_1, j_2)(n_1, n_2)}^{\infty} \Sigma_{(m_1, m_2)(n_1, n_2)}^{\infty} \end{aligned}$$

$$A_4 = \sum_{\substack{m_k, n_k \in I_k^c \\ k=1,2}} W_{(r_1, r_2)(m_1, m_2)}^\infty W_{(j_1, j_2)(n_1, n_2)}^\infty \Sigma_{(m_1, m_2)(n_1, n_2)}^\infty$$

and  $A_2, A_3$  are defined in a similar way, where  $\Sigma^\infty$  and  $\Sigma_{(m_1, m_2)(n_1, n_2)}^\infty$  are defined in Lemma S5.1. Below we are controlling these terms one by one.

We first verify that the summation of all elements  $|\Sigma_{(m_1, m_2)(n_1, n_2)}^\infty|$  is finite via the following calculation:

$$\begin{aligned} \sum_{\substack{m_k, n_k=1 \\ k=1,2}}^\infty |\Sigma_{(m_1, m_2)(n_1, n_2)}^\infty| &= \sum_{m_1=1}^\infty \sum_{m_2=1}^\infty |\Sigma_{(m_1, m_2)(m_1, m_2)}^\infty| + \sum_{\substack{m_k, n_k=1, k=1,2 \\ (m_1, m_2) \neq (n_1, n_2)}}^\infty |\Sigma_{(m_1, m_2)(n_1, n_2)}^\infty| \\ &\lesssim \sum_{m_1=1}^\infty \sum_{m_2=1}^\infty \left( \sum_{l \neq m_1} b_{lm_2}^2 \lambda_l + \tilde{\kappa}_{m_2} \right) \lambda_{m_1} + \sum_{\substack{m_k, n_k=1, k=1,2 \\ (m_1, m_2) \neq (n_1, n_2)}}^\infty b_{m_1 m_2} b_{n_1 n_2} \lambda_{m_1} \lambda_{n_1} \\ &\lesssim \sum_{m_1=1}^\infty \sum_{m_2=1}^\infty \tilde{\kappa}_{m_2}^2 \lambda_{m_1} + \sum_{m_1=1}^\infty \sum_{m_2=1}^\infty \tilde{\kappa}_{m_2} \lambda_{m_1} + \left( \sum_{m_1=1}^\infty \sum_{m_2=1}^\infty \tilde{\kappa}_{m_2} \lambda_{m_1} \right)^2 \\ &\asymp \left( \sum_{m_1=1}^\infty m_1^{-\alpha_1} \right) \left( \sum_{m_2=1}^\infty m_2^{-2\alpha_2} \right) + \left( \sum_{m_1=1}^\infty m_1^{-\alpha_1} \right) \left( \sum_{m_2=1}^\infty m_2^{-\alpha_2} \right) + \left( \sum_{m_1=1}^\infty m_1^{-\alpha_1} \right)^2 \left( \sum_{m_2=1}^\infty m_2^{-2\alpha_2} \right) \\ &< \infty. \end{aligned}$$

For  $A$ , since  $1 - a_n \lesssim W_{rr} \lesssim 1 + a_n$ , we have  $A \lesssim (1 + a_n)^2 \Sigma_{rj} - \Sigma_{rj} \lesssim a_n$  and  $A \gtrsim (1 - a_n)^2 \Sigma_{rj} - \Sigma_{rj} \gtrsim -a_n$ . This shows  $|A| \lesssim a_n$ .

For  $A_0$ , we either have  $m \neq r$  or  $n \neq j$  for each term in the summation. Therefore, the order of  $|W_{rm}|$  or  $|W_{jn}|$  is bounded by  $a_n$ . Consequently,  $|A_0| \lesssim a_n \sum_{k=1,2}^\infty |\Sigma_{(m_1, m_2)(n_1, n_2)}^\infty| \lesssim a_n$ .

For  $A_4$ , with Assumption 3.2-(i) and Lemma S5.2,

$$\begin{aligned} |A_4| &\leq \sum_{m_1=p_1+1}^\infty \sum_{m_2=p_2+1}^\infty \sum_{n_1=p_1+1}^\infty \sum_{n_2=p_2+1}^\infty |\Sigma_{(m_1, m_2)(n_1, n_2)}^\infty| \\ &\lesssim \sum_{m_1=p_1+1}^\infty \sum_{m_2=p_2+1}^\infty \lambda_{m_1} \tilde{\kappa}_{m_2} + \sum_{m_1=p_1+1}^\infty \sum_{m_2=p_2+1}^\infty \sum_{n_1=p_1+1}^\infty \sum_{n_2=p_2+1}^\infty \lambda_{m_1} \tilde{\kappa}_{m_2} \lambda_{n_1} \tilde{\kappa}_{n_2} \\ &\lesssim \left( \sum_{m_1=p_1+1}^\infty m_1^{-\alpha_1} \right) \left( \sum_{m_2=p_2+1}^\infty m_2^{-\alpha_2} \right) + \left( \sum_{m_1=p_1+1}^\infty m_1^{-\alpha_1} \right)^2 \left( \sum_{m_2=p_2+1}^\infty m_2^{-\alpha_2} \right)^2 \\ &\leq \left( \int_{p_1}^\infty x^{-\alpha_1} \right) \left( \int_{p_2}^\infty x^{-\alpha_2} \right) + \left( \int_{p_1}^\infty x^{-\alpha_1} \right)^2 \left( \int_{p_2}^\infty x^{-\alpha_2} \right)^2 \\ &= \frac{p_1^{1-\alpha_1}}{\alpha_1 - 1} \frac{p_2^{1-\alpha_2}}{\alpha_2 - 1} + \left( \frac{p_1^{1-\alpha_1}}{\alpha_1 - 1} \frac{p_2^{1-\alpha_2}}{\alpha_2 - 1} \right)^2 \\ &\lesssim p^{1-\underline{\alpha}}, \end{aligned}$$

where  $p = p_1 p_2$  and  $\underline{\alpha} = \min\{\alpha_1, \alpha_2\} > 1$ .

For  $A_1$ , we analyze one of its terms; the other terms can be bounded in a similar fashion. Observe

$$\begin{aligned}
& \sum_{\substack{m_1 \in I_1^c, n_1 \in I_1 \\ m_2, n_2 \in I_2}} |W_{(r_1, r_2)(m_1, m_2)}^\infty W_{(j_1, j_2)(n_1, n_2)}^\infty \Sigma_{(m_1, m_2)(n_1, n_2)}^\infty| \\
&= \sum_{m_1=p_1+1}^\infty \sum_{m_2=1}^{p_2} \sum_{n_1=1}^{p_1} \sum_{n_2=1}^{p_2} |\langle \tilde{\phi}_{r_1}, \phi_{m_1} \rangle \langle \tilde{\psi}_{r_2}, \psi_{m_2} \rangle \langle \tilde{\phi}_{j_1}, \phi_{n_1} \rangle \langle \tilde{\psi}_{j_2}, \psi_{n_2} \rangle \Sigma_{(m_1, m_2)(n_1, n_2)}^\infty| \\
&= \sum_{m_1 \in I_1^c} \sum_{\substack{n_1 \in I_1, m_2, n_2 \in I_2 \\ m_2 \neq r_2 \vee n_1 \neq j_1 \vee n_2 \neq j_2}} |\langle \tilde{\phi}_{r_1}, \phi_{m_1} \rangle \langle \tilde{\psi}_{r_2}, \psi_{m_2} \rangle \langle \tilde{\phi}_{j_1}, \phi_{n_1} \rangle \langle \tilde{\psi}_{j_2}, \psi_{n_2} \rangle \Sigma_{(m_1, m_2)(n_1, n_2)}^\infty| \\
&\quad + \sum_{m_1 \in I_1^c} |\langle \tilde{\phi}_{r_1}, \phi_{m_1} \rangle \langle \tilde{\psi}_{r_2}, \psi_{r_2} \rangle \langle \tilde{\phi}_{j_1}, \phi_{j_1} \rangle \langle \tilde{\psi}_{j_2}, \psi_{j_2} \rangle \Sigma_{(m_1, r_2)(j_1, j_2)}^\infty| \\
&\lesssim a_n \sum_{\substack{m_k, n_k=1 \\ k=1,2}}^\infty |\Sigma_{(m_1, m_2)(n_1, n_2)}^\infty| + \sum_{m_1=p_1+1}^\infty |\Sigma_{(m_1, r_2)(j_1, j_2)}^\infty| \\
&\lesssim a_n + p_1^{1-\alpha_1}.
\end{aligned}$$

This yields  $|A_1| \lesssim a_n + b_n$  for  $b_n = \max\{p_1^{1-\alpha_1}, p_2^{1-\alpha_2}\}$ . Similarly, one can show  $|A_2| + |A_3| \lesssim a_n + b_n$ . Combining the above bounds for  $A$  and  $A_1, \dots, A_4$ , we conclude that  $\|\tilde{\Sigma} - \Sigma\|_\infty \lesssim a_n + b_n$ .

Finally, if  $d_{\mathcal{X}} < \infty$  and  $d_{\mathcal{Y}} < \infty$ , there will be no tail sum parts in the above summations  $A_k, k = 0, \dots, 4$ . Hence, all the  $A$ 's can be upper bounded by the order of  $a_n$ , which gives the second result.  $\square$

The following proposition states the relation between the corresponding test sequences induced by different pairs of bases of  $\mathcal{X}$  and  $\mathcal{Y}$ . Recall in Section 2, we consider the dimensions of  $\mathcal{X}$  and  $\mathcal{Y}$  to be  $d_{\mathcal{X}}$  and  $d_{\mathcal{Y}}$  respectively, with  $d_{\mathcal{X}}$  or  $d_{\mathcal{Y}}$  being finite or infinite. To simplify notations, we only consider the case with  $d_{\mathcal{X}} = \infty$  and  $d_{\mathcal{Y}} = \infty$ ; analysis for other cases with finite dimensions of  $\mathcal{X}$  or  $\mathcal{Y}$  is similar.

**Proposition S5.4.** *For orthonormal bases  $\{\tilde{\phi}_{j_1}\}_{j_1=1}^\infty$  and  $\{\tilde{\psi}_{j_2}\}_{j_2=1}^\infty$  of  $\mathcal{X}$  and  $\mathcal{Y}$  respectively, and the corresponding sequence  $V_i^\infty(\tilde{\phi}, \tilde{\psi}) = (\tilde{\xi}_{ij_1}, \tilde{\zeta}_{ij_2}, j_1, j_2 = 1, \dots)$ , where  $\tilde{\xi}_{ij_1} = \langle X_i, \tilde{\phi}_{j_1} \rangle$ ,  $\tilde{\zeta}_{ij_2} = \langle Y_i, \tilde{\psi}_{j_2} \rangle$ , there is a unitary operator  $W(\tilde{\phi}, \tilde{\psi})$  on  $\ell^2 \times \ell^2$  such that*

$$V_i^\infty(\tilde{\phi}, \tilde{\psi}) = W^\dagger(\tilde{\phi}, \tilde{\psi}) V_i^\infty(\phi, \psi),$$

where  $V_1^\infty(\phi, \psi)$  is defined before Assumption 3.1 and  $W^\dagger$  is the adjoint of  $W$ .

*Proof.* For  $X$ , given  $\{\phi_j\}_{j=1}^\infty$  and  $\{\tilde{\phi}_j\}_{j=1}^\infty$ , define maps  $T_{\mathcal{X}}, \tilde{T}_{\mathcal{X}} : \mathcal{X} \rightarrow \ell^2$  by

$$\begin{aligned}
T_{\mathcal{X}} : X &\mapsto (\langle X, \phi_j \rangle)_{j=1}^\infty, \\
\tilde{T}_{\mathcal{X}} : X &\mapsto (\langle X, \tilde{\phi}_j \rangle)_{j=1}^\infty.
\end{aligned}$$

It is seen that these two maps are well-defined and onto  $\ell^2$ . Moreover, they are unitary. Let  $F_{X,i}^\infty = (\langle X_i, \phi_j \rangle)_{j=1}^\infty$  and  $\tilde{F}_{X,i}^\infty = (\langle X_i, \tilde{\phi}_j \rangle)_{j=1}^\infty$  be the Fourier coefficients of  $X_i$  w.r.t  $\{\phi_j\}_{j=1}^\infty$  and  $\{\tilde{\phi}_j\}_{j=1}^\infty$ , respectively.

From the fact that  $T_{\mathcal{X}}$  and  $\tilde{T}_{\mathcal{X}}$  are unitary and  $T_{\mathcal{X}}^{\dagger}F_{X,i}^{\infty} = X = \tilde{T}_{\mathcal{X}}^{\dagger}\tilde{F}_{X,i}^{\infty}$ , we have

$$\tilde{F}_{X,i}^{\infty} = U_{\mathcal{X}}^{\dagger}F_{X,i}^{\infty},$$

where  $U_{\mathcal{X}}^{\dagger}$  is the adjoint operator of the unitary operator  $U_{\mathcal{X}} = T_{\mathcal{X}}\tilde{T}_{\mathcal{X}}^{\dagger}$ , the composition of  $T_{\mathcal{X}}$  and  $\tilde{T}_{\mathcal{X}}^{\dagger}$ . Similarly, for  $Y$ , with the similar definitions and notations, we have

$$\tilde{F}_{Y,i}^{\infty} = U_{\mathcal{Y}}^{\dagger}F_{Y,i}^{\infty},$$

for the unitary operator  $U_{\mathcal{Y}} = T_{\mathcal{Y}}\tilde{T}_{\mathcal{Y}}^{\dagger}$ .

Define  $W(\tilde{\phi}, \tilde{\psi}) \triangleq U_{\mathcal{X}} \otimes U_{\mathcal{Y}}$ , whose definition follows from the tensor product of linear maps, as an operator on  $\ell^2 \times \ell^2$ . It is easy to check that  $W(\tilde{\phi}, \tilde{\psi})$  is unitary with  $W^{\dagger}(\tilde{\phi}, \tilde{\psi}) = U_{\mathcal{X}}^{\dagger} \otimes U_{\mathcal{Y}}^{\dagger}$  as its adjoint operator. Therefore, we have

$$\tilde{V}_i^{\infty} = \tilde{F}_{X,i}^{\infty} \otimes \tilde{F}_{Y,i}^{\infty} = U_{\mathcal{X}}^{\dagger}F_{X,i}^{\infty} \otimes U_{\mathcal{Y}}^{\dagger}F_{Y,i}^{\infty} = (U_{\mathcal{X}}^{\dagger} \otimes U_{\mathcal{Y}}^{\dagger})(F_{X,i}^{\infty} \otimes F_{Y,i}^{\infty}) = W^{\dagger}(\tilde{\phi}, \tilde{\psi})V_i^{\infty}.$$

□

## S6 Proof of Proposition 2.1

*Proof.* By expansion (6), the FLM (1) in Section 1 can be written as

$$Y = \sum_{j_1=1}^{\infty} \sum_{j_2=1}^{\infty} b_{j_1 j_2} \langle X, \phi_{j_1} \rangle_1 \psi_{j_2} + Z.$$

Accordingly,

$$\begin{aligned} g &= \mathbb{E}[X \otimes Y] = \mathbb{E}\left[X \otimes \left(\sum_{j_1=1}^{\infty} \sum_{j_2=1}^{\infty} b_{j_1 j_2} \langle X, \phi_{j_1} \rangle_1 \psi_{j_2}\right)\right] \\ &= \sum_{j_1=1}^{\infty} \sum_{j_2=1}^{\infty} b_{j_1 j_2} \mathbb{E}[\langle X, \phi_{j_1} \rangle_1 X] \otimes \psi_{j_2} = \sum_{j_1=1}^{\infty} \sum_{j_2=1}^{\infty} b_{j_1 j_2} (C_X \phi_{j_1}) \otimes \psi_{j_2} \\ &= \sum_{j_1=1}^{\infty} \sum_{j_2=1}^{\infty} b_{j_1 j_2} \left(\sum_k \lambda_k \langle \phi_{j_1}, \phi_k \rangle_1 \phi_{j_1}\right) \otimes \psi_{j_2} = \sum_{j_1=1}^{\infty} \sum_{j_2=1}^{\infty} b_{j_1 j_2} \lambda_{j_1} \phi_{j_1} \otimes \psi_{j_2}. \end{aligned}$$

Given the above, we find that

$$\begin{aligned} g_{j_1 j_2} &= \langle g, \phi_{j_1} \otimes \psi_{j_2} \rangle = \sum_{n=1}^{\infty} \sum_{m=1}^{\infty} b_{mn} \lambda_m \langle \phi_m \otimes \psi_n, \phi_{j_1} \otimes \psi_{j_2} \rangle \\ &= \sum_{n=1}^{\infty} \sum_{m=1}^{\infty} b_{mn} \lambda_m \langle \phi_m, \phi_{j_1} \rangle_1 \langle \psi_n, \psi_{j_2} \rangle_2 = \lambda_j b_{j_1 j_2}, \end{aligned}$$

which shows that  $b_{j_1 j_2} = \lambda_{j_1}^{-1} g_{j_1 j_2}$ . By Fubini's Theorem,  $g_{j_1 j_2} = \langle g, \phi_{j_1} \otimes \psi_{j_2} \rangle = \langle \mathbb{E}[X \otimes Y], \phi_{j_1} \otimes \psi_{j_2} \rangle = \mathbb{E}[\langle X \otimes Y, \phi_{j_1} \otimes \psi_{j_2} \rangle] = \mathbb{E}[\langle X, \phi_{j_1} \rangle_1 \langle Y, \psi_{j_2} \rangle_2]$ .  $\square$

## S7 Proof of Proposition 3.4

*Proof.* Recall the Karhunen–Loève expansion of the covariance operator  $C_X = \mathbb{E}[X \otimes X] = \sum_{j=1}^{d_X} \lambda_j \phi_j \otimes \phi_j$ . Define  $P_r = \phi_r \otimes \phi_r$  and its empirical version  $\hat{P}_r = \hat{\phi}_r \otimes \hat{\phi}_r$ . Let  $g_{1,r} := \lambda_r - \lambda_{r-1}$  for  $r \geq 1$ , and  $\bar{g}_{1,r} := \min\{g_{1,r-1}, g_{1,r}\}$  for  $r \geq 2$  with  $\bar{g}_{1,1} = g_{1,1}$ . Since we assume that  $\lambda_j \asymp j^{-\alpha_1}$  for some  $\alpha_1 > 2$ , the effective rank

$$\mathbf{r}(C_X) = \frac{\text{tr}(C_X)}{\|C_X\|_2},$$

of the covariance operator  $C_X$  is always bounded, where  $\text{tr}(C_X)$  and  $\|C_X\|_2$  are respectively the trace and the operator norm of the operator  $C_X$ . Moreover,  $\bar{g}_{1,r} \asymp r^{-(\alpha_1+1)} \geq p_1^{-(\alpha_1+1)}$ , and  $\|C_X\|_2$  is bounded.

Similar to the results in Koltchinskii et al. (2016), under our setting, from Proposition S8.4, we have with probability at least  $1 - e^{-t}$ ,

$$|\langle (\hat{P}_r - P_r)u, v \rangle| \lesssim \frac{1}{\bar{g}_{1,r}} \sqrt{\frac{t}{n}} \|u\| \|v\|,$$

for  $u, v \in \mathcal{X}$ . Hence, for  $j \neq r$ , taking  $u = \hat{\phi}_j$  and  $v = -\phi_r$ , we have

$$\langle (\hat{P}_r - P_r)u, v \rangle = \langle (\hat{P}_r - P_r)\hat{\phi}_j, -\phi_r \rangle = \langle \phi_r, \hat{\phi}_j \rangle.$$

In addition, for  $j = r$ , taking  $u = \hat{\phi}_r$  and  $v = \hat{\phi}_r$ , we have

$$\langle (\hat{P}_r - P_r)u, v \rangle = \langle (\hat{P}_r - P_r)\hat{\phi}_r, \hat{\phi}_r \rangle = 1 - \langle \phi_r, \hat{\phi}_r \rangle^2.$$

These imply that, for  $j \neq r$ , with probability at least  $1 - e^{-t}$ ,

$$|\langle \phi_r, \hat{\phi}_j \rangle| \lesssim \frac{1}{\bar{g}_{1,r}} \sqrt{\frac{t}{n}}.$$

For  $j = r$ , we observe

$$\begin{aligned} |\langle \phi_r, \hat{\phi}_r \rangle - 1| &= \left| \sqrt{1 - \langle (\hat{P}_r - P_r)\hat{\phi}_r, \hat{\phi}_r \rangle} - 1 \right| \\ &\lesssim \max \left\{ \sqrt{1 + \frac{1}{\bar{g}_{1,r}} \sqrt{\frac{t}{n}}} - 1, 1 - \sqrt{1 - \frac{1}{\bar{g}_{1,r}} \sqrt{\frac{t}{n}}} \right\} \\ &= 1 - \sqrt{1 - \frac{1}{\bar{g}_{1,r}} \sqrt{\frac{t}{n}}} \asymp \frac{1}{\bar{g}_{1,r}} \sqrt{\frac{t}{n}}, \end{aligned}$$

with probability at least  $1 - e^{-t}$ . Similarly, for the transformation matrix  $U_Y^p(\hat{\psi})$  defined in Section 3, we

have

$$\begin{aligned} |\langle \psi_r, \hat{\psi}_j \rangle| &\lesssim \frac{1}{\bar{g}_{2,r}} \sqrt{\frac{t}{n}} & j \neq r, \\ |\langle \psi_r, \hat{\psi}_r \rangle - 1| &\lesssim \frac{1}{\bar{g}_{2,r}} \sqrt{\frac{t}{n}} & j = r, \end{aligned}$$

with probability at least  $1 - e^{-t}$  for  $\bar{g}_{2,r} \geq p_2^{-(\alpha_2+1)}$ , where  $\bar{g}_{2,r}$  is defined in analogy to  $\bar{g}_{1,r}$  by replacing  $\{\lambda_j\}_{j=1}^{p_1}$  with  $\{\rho_j\}_{j=1}^{p_2}$ .

Note that for  $W := W_p(\hat{\phi}, \hat{\psi}) = U_{\mathcal{X}}^p(\hat{\phi}) \otimes U_{\mathcal{Y}}^p(\hat{\psi})$ , we have  $W_{ij} = \langle \phi_{i_1}, \hat{\phi}_{j_1} \rangle \langle \psi_{i_2}, \hat{\psi}_{j_2} \rangle$ , where  $i = p_1(i_2 - 1) + i_1$  and  $j = p_1(j_2 - 1) + j_1$ . Let  $\tilde{a}_{n,1} = \frac{1}{\bar{g}_{1,r}} \sqrt{\frac{t}{n}}$  and  $\tilde{a}_{n,2} = \frac{1}{\bar{g}_{2,r}} \sqrt{\frac{t}{n}}$  with suitable  $t$  such that  $\frac{t}{n} = o_n(1)$ . Below we divide the proof into three cases.

- $j_1 = i_1$  and  $j_2 = i_2$ , which implies  $j = i$ . Since  $|\langle \phi_{i_1}, \hat{\phi}_{i_1} \rangle - 1| \lesssim \tilde{a}_{n,1}$  with probability at least  $1 - e^{-t}$  and  $|\langle \psi_{i_2}, \hat{\psi}_{i_2} \rangle - 1| \lesssim \tilde{a}_{n,2}$  with probability at least  $1 - e^{-t}$ , we have  $(1 - \tilde{a}_{n,1})(1 - \tilde{a}_{n,2}) \lesssim \langle \phi_{i_1}, \hat{\phi}_{i_1} \rangle \langle \psi_{i_2}, \hat{\psi}_{i_2} \rangle \lesssim (1 + \tilde{a}_{n,1})(1 + \tilde{a}_{n,2})$  with probability at least  $(1 - e^{-t})^2$ . That is, there is a constant  $C > 0$  such that

$$C[\tilde{a}_{n,1}\tilde{a}_{n,2} - (\tilde{a}_{n,1} + \tilde{a}_{n,2})] \leq W_{ii} - 1 \leq C[\tilde{a}_{n,1}\tilde{a}_{n,2} + (\tilde{a}_{n,1} + \tilde{a}_{n,2})],$$

which further implies that

$$|W_{ii} - 1| \leq C \max\{\tilde{a}_{n,1}, \tilde{a}_{n,2}\} = C \max\left\{\frac{1}{\bar{g}_{1,r}}, \frac{1}{\bar{g}_{2,r}}\right\} \sqrt{\frac{t}{n}},$$

with probability at least  $(1 - e^{-t})^2 > 1 - 2e^{-t}$ . By adjusting the constant  $C$ , we can replace  $1 - 2e^{-t}$  by  $1 - e^{-t}$ .

- $j_1 \neq i_1$  and  $j_2 \neq i_2$ . In this case, we have

$$|W_{ij}| \lesssim \frac{1}{\bar{g}_{1,r}\bar{g}_{2,r}} \frac{t}{n} \leq \max\left\{\frac{1}{\bar{g}_{1,r}}, \frac{1}{\bar{g}_{2,r}}\right\} \sqrt{\frac{t}{n}},$$

with probability at least  $1 - e^{-t}$ .

- $j_1 = i_1$  and  $j_2 \neq i_2$ ; the case of  $j_1 \neq i_1$  and  $j_2 = i_2$  is analyzed in a similar fashion. We have

$$(1 - \tilde{a}_{n,1})\tilde{a}_{n,2} \lesssim m_{i_1 i_1} \tilde{m}_{i_2 j_2} \lesssim (1 + \tilde{a}_{n,1})\tilde{a}_{n,2},$$

which further implies that

$$|W_{ij}| \lesssim \tilde{a}_{n,2} \leq \max\left\{\frac{1}{\bar{g}_{1,r}}, \frac{1}{\bar{g}_{2,r}}\right\} \sqrt{\frac{t}{n}},$$

with probability at least  $1 - e^{-t}$ . In addition,

$$|W_{ij}| \lesssim \tilde{a}_{n,1} \leq \max\left\{\frac{1}{\bar{g}_{1,r}}, \frac{1}{\bar{g}_{2,r}}\right\} \sqrt{\frac{t}{n}},$$

with probability at least  $1 - e^{-t}$ .

Let  $a_{n,t} = \max\{p_1^{\alpha_1+1}, p_2^{\alpha_2+1}\} \sqrt{t/n} > 0$  with a suitable  $t$  such that  $a_{n,t} = o_n(1)$ . Then we conclude that

$$\begin{aligned} \mathbb{P}(\|W - I_p\|_\infty \gtrsim a_{n,t}) &= \mathbb{P}\left(\bigcup_{r,j} \{|W_{rj} - (I_p)_{rj}| \gtrsim a_{n,t}\}\right) \\ &\leq \sum_{r,j} \mathbb{P}(|W_{rj} - (I_p)_{rj}| \gtrsim a_{n,t}) \\ &\leq \sum_{r,j} \mathbb{P}\left(|W_{rj} - (I_p)_{rj}| \gtrsim \max\left\{\frac{1}{\bar{g}_{1,r}}, \frac{1}{\bar{g}_{2,r}}\right\} \sqrt{\frac{t}{n}}\right) \\ &\leq \sum_{r,j} e^{-t} \leq e^{-t+2\ln p}, \end{aligned}$$

which is equivalent to  $\|W - I_p\|_\infty \lesssim a_{n,t}$  with probability at least  $1 - e^{-t+2\ln p}$ .  $\square$

## S8 A Concentration Inequality for $\langle \phi_r, \hat{\phi}_j \rangle$

The proof of Proposition 3.4 depends on Proposition S8.4 to be stated below, which in turn depends on the following lemmas from Koltchinskii et al. (2016).

**Lemma S8.1.** *Let  $X, X_1, \dots, X_n$  be i.i.d. centered sub-Gaussian random vectors in a Hilbert space with covariance  $C_X = \mathbb{E}(X \otimes X)$ . For all  $p \geq 1$ ,*

$$\mathbb{E}^{1/p} \|\hat{C}_X - C_X\|_2^p \asymp \|C_X\|_2 \max\left\{\sqrt{\frac{\mathbf{r}(C_X)}{n}}, \frac{\mathbf{r}(C_X)}{n}\right\}.$$

**Lemma S8.2.** *Let  $X, X_1, \dots, X_n$  be i.i.d. centered sub-Gaussian random vectors in a Hilbert space with covariance  $C_X = \mathbb{E}(X \otimes X)$ . There exist a constant  $C_1 > 0$  such that for all  $t \geq 1$  with probability at least  $1 - e^{-t}$ ,*

$$\|\hat{C}_X - C_X\|_2 \leq C_1 \|C_X\|_2 \left[ \sqrt{\frac{\mathbf{r}(C_X)}{n}} \vee \frac{\mathbf{r}(C_X)}{n} \vee \sqrt{\frac{t}{n}} \vee \frac{t}{n} \right].$$

Let  $E = \hat{C}_X - C_X$  and  $\bar{g}_r = \bar{g}_{1,r}$  as in the proof of Proposition 3.4. Denote

$$O_r = \sum_{s \neq r} \frac{1}{\lambda_r - \lambda_s} P_s,$$

with  $P_s = \phi_s \otimes \phi_s$ .

**Lemma S8.3.** *It holds that*

$$\|\hat{P}_r - P_r\|_2 \leq 4 \frac{\|E\|_2}{\bar{g}_r}.$$

Moreover,  $\hat{P}_r - P_r = L_r(E) + S_r(E)$ , where  $L_r(E) = O_r E P_r + P_r E C_r$  and  $\|S_r(E)\|_2 \leq 14 \left( \frac{\|E\|_2}{\bar{g}_r} \right)^2$ .

*Remark 1.* Although Lemma S8.1 and Lemma S8.2 in Koltchinskii et al. (2016) are stated for Gaussian elements, Remark 1 therein mentions that such results also hold for centered sub-Gaussian elements. Also, the Lemma S8.3 is without a Gaussian assumption.

Now we are ready to state and prove the proposition.

**Proposition S8.4.** *Let  $X, X_1, \dots, X_n$  be i.i.d. centered sub-Gaussian random vectors in a separable Hilbert space  $\mathcal{X}$  with covariance  $C_X = \mathbb{E}(X \otimes X)$ . If Assumptions 3.1–3.2 hold, then with probability at least  $1 - e^{-t}$  for  $t > 0$ , we have*

$$|\langle (\hat{P}_r - P_r)u, v \rangle| \lesssim \frac{1}{\bar{g}_{1,r}} \sqrt{\frac{t}{n}} \|u\| \|v\|,$$

for  $u, v \in \mathcal{X}$ .

*Proof.* It is seen that

$$\begin{aligned} |\langle (\hat{P}_r - P_r)u, v \rangle| &= |\langle (\hat{P}_r - \mathbb{E}\hat{P}_r)u, v \rangle| + |\langle (\mathbb{E}\hat{P}_r - P_r)u, v \rangle| \\ &\leq |\langle (\hat{P}_r - \mathbb{E}\hat{P}_r)u, v \rangle| + \|\mathbb{E}\hat{P}_r - P_r\|_2 \|u\| \|v\|, \end{aligned}$$

where  $\|u\|$  denotes the norm of  $u$  in  $\mathcal{X}$ . As in Corollary 1 and Theorem 4 of Koltchinskii et al. (2016), it remains to bound  $|\langle (\hat{P}_r - \mathbb{E}\hat{P}_r)u, v \rangle|$  and  $\|\mathbb{E}\hat{P}_r - P_r\|_2$ . In the sequel, we use  $D$  to denote a constant whose value may vary in different places. It is sufficient to consider the case with large enough  $n$  and bounded  $\mathbf{r}(C_X)$ .

From Lemma S8.3,  $\hat{P}_r - P_r = L_r(E) + S_r(E)$ , where  $L_r(E) = O_r E P_r + P_r E C_r$  and  $E = \hat{C}_X - C_X$ . In addition,  $\mathbb{E}L_r(E) = 0$  due to  $\mathbb{E}E = 0$ . Then we have

$$\begin{aligned} \|\mathbb{E}\hat{P}_r - P_r\|_2 &= \|\mathbb{E}(\hat{P}_r - P_r)\|_2 = \|\mathbb{E}(L_r(E) + S_r(E))\|_2 \\ &= \|\mathbb{E}S_r(E)\|_2 \leq \mathbb{E}\|S_r(E)\|_2 \\ &\leq D \frac{\mathbb{E}\|E\|_2^2}{\bar{g}_r^2} \lesssim \frac{\|\Sigma\|_2^2 \mathbf{r}(\Sigma)}{\bar{g}_r^2 n}, \end{aligned}$$

where the last line is based on Lemma S8.1.

Now we analyze the term  $|\langle (\hat{P}_r - \mathbb{E}\hat{P}_r)u, v \rangle|$ . As in Lemma S8.3, let  $R_r = (\hat{P}_r - P_r) - \mathbb{E}(\hat{P}_r - P_r) - L_r = \hat{P}_r - \mathbb{E}\hat{P}_r - L_r$ . Then,

$$|\langle (\hat{P}_r - \mathbb{E}\hat{P}_r)u, v \rangle| \leq |\langle R_r u, v \rangle| + |\langle L_r u, v \rangle|.$$

According to a discussion after Theorem 3 of Koltchinskii et al. (2016),  $\langle L_r u, v \rangle$  can be written as a sum of i.i.d. sub-exponential random variables with the assumption that  $X_i$  are sub-Gaussian random elements.

By using a Bernstein inequality we then have

$$|\langle L_r u, v \rangle| \leq D_1 \frac{\|C_X\|_2}{\bar{g}_r} \sqrt{\frac{t}{n}} \|u\| \|v\| \quad (\text{S32})$$

with probability at least  $1 - e^{-t}$ .

To bound the term  $|\langle R_r u, v \rangle|$ , without loss of generality, assume  $\|u\| \leq 1$  and  $\|v\| \leq 1$ . First, we observe that

$$R_r = S_r(E) - \mathbb{E}S_r(E),$$

and

$$|\langle S_r(E)u, v \rangle| \leq \|S_r(E)\|_2 \leq \|\hat{P}_r - P_r\|_2 + \|L_r(E)\|_2 \leq \|\hat{P}_r - P_r\|_2 + 2 \frac{\|E\|_2}{\bar{g}_r} \leq 6 \frac{\|E\|_2}{\bar{g}_r}.$$

Then, we use Lemma S8.2 to derive that, with probability at least  $1 - e^{-t}$ ,

$$|\langle S_r(E)u, v \rangle| \lesssim \frac{\|C_X\|_2}{\bar{g}_r} \left( \sqrt{\frac{\mathbf{r}(C_X)}{n}} \vee \frac{\mathbf{r}(C_X)}{n} \vee \sqrt{\frac{t}{n}} \vee \frac{t}{n} \right).$$

By taking  $t = \log 2$ , we see that  $1 - e^{-t} = 1/2$  and consequently observe that

$$\text{Med} \lesssim \frac{\|C_X\|_2}{\bar{g}_r} \left( \sqrt{\frac{\mathbf{r}(C_X)}{n}} \vee \frac{\mathbf{r}(C_X)}{n} \vee \sqrt{\frac{1}{n}} \vee \frac{1}{n} \right),$$

where Med is the median of  $|\langle S_r(E)u, v \rangle|$ . This implies that, all  $t \geq 1$ , with probability at least  $1 - e^{-t}$ ,

$$|\langle S_r(E)u, v \rangle - \text{Med}| \lesssim \frac{\|C_X\|_2}{\bar{g}_r} \left( \sqrt{\frac{\mathbf{r}(C_X)}{n}} \vee \frac{\mathbf{r}(C_X)}{n} \vee \sqrt{\frac{t}{n}} \vee \frac{t}{n} \right).$$

Integrating the tail of this exponential bound yields that, for some  $D'_2 > 0$ ,

$$|\mathbb{E}\langle S_r(E)u, v \rangle - \text{Med}| \leq \mathbb{E}|\langle S_r(E)u, v \rangle - \text{Med}| \leq D'_2 \frac{\|C_X\|_2}{\bar{g}_r} \left( \sqrt{\frac{\mathbf{r}(C_X)}{n}} \vee \frac{\mathbf{r}(C_X)}{n} \vee \sqrt{\frac{1}{n}} \vee \frac{1}{n} \right),$$

which in turn implies that one can replace Med by the expectation  $\mathbb{E}\langle S_r(E)u, v \rangle$  in the concentration bound to conclude that, with some  $D_2 > 0$  and with probability at least  $1 - 2e^{-t}$ ,

$$|\langle R_r u, v \rangle| = |\langle S_r(E)u, v \rangle - \mathbb{E}\langle S_r(E)u, v \rangle| \leq D_2 \frac{\|C_X\|_2}{\bar{g}_r} \left( \sqrt{\frac{\mathbf{r}(C_X)}{n}} \vee \frac{\mathbf{r}(C_X)}{n} \vee \sqrt{\frac{t}{n}} \vee \frac{t}{n} \right), \quad (\text{S33})$$

where by adjusting the constant  $D_2$  one can replace  $1 - 2e^{-t}$  by  $1 - e^{-t}$ .

Combining (S32) and (S33) with suitable constants  $D_1$  and  $D_2$  yields

$$|\langle (\hat{P}_r - \mathbb{E}P_r)u, v \rangle| \leq D_1 \frac{\|C_X\|_2}{\bar{g}_r} \sqrt{\frac{t}{n}} \|u\| \|v\| + D_2 \frac{\|C_X\|_2}{\bar{g}_r} \left( \sqrt{\frac{\mathbf{r}(C_X)}{n}} \vee \frac{\mathbf{r}(C_X)}{n} \vee \sqrt{\frac{t}{n}} \vee \frac{t}{n} \right) \|u\| \|v\|,$$

with probability at least  $1 - e^{-t}$ . With the bounded  $\mathbf{r}(C_X)$  and  $\|C_X\|_2$ ,  $t = O(n)$  and  $\frac{t}{n} = o(n)$ , we conclude that, with high probability,

$$|(\hat{P}_r - \mathbb{E}P_r)u, v| \lesssim \frac{1}{\bar{g}_r} \sqrt{\frac{t}{n}} \|u\| \|v\|,$$

which leads to

$$|(\hat{P}_r - P_r)u, v| \lesssim \frac{1}{\bar{g}_r} \sqrt{\frac{t}{n}} \|u\| \|v\| + \frac{1}{\bar{g}_r^2 n} \|u\| \|v\| \lesssim \frac{1}{\bar{g}_r} \sqrt{\frac{t}{n}} \|u\| \|v\|,$$

with  $\frac{1}{\bar{g}_r} \sqrt{\frac{t}{n}} = o(n)$ . □

*Remark 2.* It can be shown that if  $X$  and  $Z$  in (1) are sub-Gaussian random elements in  $\mathcal{X}$  and  $\mathcal{Y}$ , respectively, then  $Y$  from (1) is also a sub-Gaussian random variable in  $\mathcal{Y}$ . Proposition S8.4 then hold also for  $Y$ , which is needed in the proof of Proposition 3.4.

## References

- Koltchinskii, V., Lounici, K., et al. (2016), “Asymptotics and concentration bounds for bilinear forms of spectral projectors of sample covariance,” in *Annales de l’Institut Henri Poincaré, Probabilités et Statistiques*, Institut Henri Poincaré, vol. 52, pp. 1976–2013.
- Lin, Z., Lopes, M. E., and Müller, H.-G. (2022), “High-dimensional MANOVA via Bootstrapping and its Application to Functional Data and Sparse Count Data,” *Journal of the American Statistical Association*, to appear.
- Lopes, M. E., Lin, Z., and Müller, H.-G. (2020), “Bootstrapping max statistics in high dimensions: Near-parametric rates under weak variance decay and application to functional data analysis,” *The Annals of Statistics*, 48, 1214–1229.
- Lopes, M. E. and Yao, J. (2022), “A sharp lower-tail bound for Gaussian maxima with application to bootstrap methods in high dimensions,” *Electronic Journal of Statistics*, 16, 58–83.
- Pollard, D. (1990), “Empirical processes: theory and applications,” in *NSF-CBMS regional conference series in probability and statistics*, JSTOR, pp. i–86.
- Shalev-Shwartz, S. and Ben-David, S. (2014), *Understanding machine learning: From theory to algorithms*, Cambridge university press.
- Vershynin, R. (2018), *High-dimensional probability: An introduction with applications in data science*, vol. 47, Cambridge university press.
